# Supplementary material for: Provably Efficient Cooperative Multi-Agent Reinforcement Learning with Function Approximation
Source: arXiv:2103.04972 source file (2021-03-08)
Supplement: Supplementary file 1 [file appendix_federated.tex]

\section{Proofs for Parallel MDPs}
\subsection{Proof for Homogenous Regret (Theorem~\ref{thm:ind_homo})}
We first restate the Theorem for completeness.

\textbf{Theorem}.
\textbf{\texttt{CoopLSVI}} when run on $M$ agents with communication threshold $S$, $\beta_t = \cO(H\sqrt{\log tMH})$ and $\lambda = 1 - (MTH)^{-1}$ obtains the following cumulative regret after $T$ episodes, with probability at least $1-\alpha$,
\begin{align*}
\regret(T)=\widetilde\cO\left(H^2\left(M\sqrt{S} + \sqrt{MT}\right)\sqrt{\log\left(\frac{1}{\alpha}\right)}\right).
\end{align*}

\begin{proof}
Observe that the group regret at any instant $T$ can be given as follows.
\begin{align}
    \regret(T) = \sum_{t=1}^T\sum_{m=1}^M \left[V^\star_1(x^1_{m, h}) - V^{\pi^t_m}_1(x^1_{m, h}) \right].
\end{align}
Let $\delta^t_h(\bz) = \sum_{m=1}^M \left[r_{m, h}(z_m) + \bbP_{m, h}V^t_{m, h+1}(z_m) - Q^t_{m, h}(z_m)\right]$ denote the temporal-difference (TD) error of any parallel multi-agent setting for the state-action pair $\bz$. We additionally define $\xi^1_{t, m, h}$ and $\xi^2_{t, m, h} \in \bbR$ as follows.
\begin{align}
    \xi^1_{t, m, h} &= \left[V^t_{m, h}(x^t_{m, h}) - V^{\pi^t_m}_{m, h}(x^t_{m, h})\right] - \left[ Q^t_{m, h}(x^t_{m, h}, a^t_{m, h}) - Q^{\pi^t_m}_{m, h}(x^t_{m, h}, a^t_{m, h}) \right], \\
    \xi^2_{t, m, h} &= \left[\bbP_{m, h}V^t_{m, h+1}(x^t_{m, h}, a^t_{m, h}) - \bbP_{m, h}V^{\pi^t_m}_{m, h+1}(x^t_{m, h}, a^t_{m, h})\right]
    - \left[ V^t_{m, h}(x^t_{m, h+1}) - V^{\pi^t_m}_{m, h}(x^t_{m, h+1}) \right].
\end{align}
For each agent, $\xi^1_{t, m, h}$ and $\xi^2_{t, m, h}$ denote the randomness of the policy and the randomness of the environments, and will form a Martingale difference sequence. Now, to bound the regret, we decompose it in terms of the above defined quantities. By Lemma~\ref{lem:regret_decomp_factored}, we have,
\begin{multline}
    \regret(T) = \underbrace{\sum_{t=1}^T\sum_{h=1}^H \left[ \bbE_{\bpi^\star}\left[ \delta^t_h(\bz) | \x_1 = \x_1^t\right] -\delta^t_h(\bz^t_h)\right]}_{\text{(A)}} + \underbrace{\sum_{t=1}^T\sum_{h=1}^H\sum_{m=1}^M \left[\xi^1_{t, m, h} + \xi^2_{t, m, h}\right]}_{\text{(B)}} \\ + \underbrace{\sum_{t=1}^T\sum_{h=1}^H\sum_{m=1}^M \bbE_{\pi^\star_m}\left[\left\langle Q^t_{m, h}(x_m, \cdot), \pi^\star_m(\cdot|x_m) - \pi^t_h(\cdot | x_m)\right\rangle_\cA | \x_1 = \x^t_1\right]}_{\text{(C)}}.
\end{multline}
Here, since $\pi^t_{m, h}$ for any agent $m$ at any instant $(t, h) \in [T]\times[H]$ is the greedy policy (with respect to $Q^t_{m, h}$), we have that, by definition,
\begin{align}
    \left\langle Q^t_{m, h}(x_m, \cdot), (\pi^\star_m - \pi^t_h)(\cdot | x_m)\right\rangle_\cA = \left\langle Q^t_{m, h}(x_m, \cdot), \pi^\star_m(\cdot|x_m)\right\rangle_\cA - \max_{a \in \cA}Q^t_{m, h}(x_m, a) \leq 0.
\end{align}
for all $x_m \in \cS$, and hence, term (C) is less than $0$. This leaves us with the following decomposition for the regret.
\begin{align}
    \regret(T) \leq \underbrace{\sum_{t=1}^T\sum_{h=1}^H \left[ \bbE_{\bpi^\star}\left[ \delta^t_h(\bz) | \x_1 = \x_1^t\right] -\delta^t_h(\bz^t_h)\right]}_{\text{(A)}} + \underbrace{\sum_{t=1}^T\sum_{h=1}^H\sum_{m=1}^M \left[\xi^1_{t, m, h} + \xi^2_{t, m, h}\right]}_{\text{(B)}}.
\end{align}
We can bound term (B) by Lemma~\ref{lem:martingale_independent}. With probability at least $1-\alpha/2$ for some $\alpha>0$,
\begin{align}
    \regret(T) \leq \sum_{t=1}^T\sum_{h=1}^H \left[ \bbE_{\bpi^\star}\left[ \delta^t_h(\bz) | \x_1 = \x_1^t\right] -\delta^t_h(\bz^t_h)\right] + \sqrt{16H^3MT\log\left(\frac{4}{\alpha}\right)}.
\end{align}
We can bound the first term by Lemma~\ref{lem:beta_independent_centralized}. First, note that $\bbE_{\bpi^\star}\left[ \delta^t_h(\bz) | \x_1 = \x_1^t\right] \geq 0$. Therefore,  
\begin{align}
    \regret(T) &\leq \sum_{t=1}^T\sum_{h=1}^H \left[ \bbE_{\bpi^\star}\left[ \delta^t_h(\bz) | \x_1 = \x_1^t\right] -\delta^t_h(\bz^t_h)\right] + \sqrt{16H^3MT\log\left(\frac{4}{\alpha}\right)} \\
    &\leq \sum_{t=1}^T\sum_{h=1}^H \left[-\delta^t_h(\bz^t_h)\right] + \sqrt{16H^3MT\log\left(\frac{4}{\alpha}\right)}.
\end{align}
To bound $-\delta^t_h(\bz^t_h)$, we have, by Lemma~\ref{lem:beta_independent_centralized} that with probability at least $1-\alpha'$ for some $\alpha' >0$,
\begin{align*}
    0 \leq -\delta^t_h(\bz) \leq 2\bar\beta^t_{h}\left(\epsilon, \frac{\alpha'}{M}\right)\left(\sum_{m=1}^M \left\lVert \bphi(z_m) \right\rVert_{(\bLambda^t_{m, h})^{-1}}\right).
\end{align*}
By a union bound and setting $\alpha = \alpha'/2TH$, we have that with probability at least $1-\alpha/2$,
\begin{align*}
    \sum_{t=1}^T\sum_{h=1}^H -\delta^t_h(\bz^t_h)
    &\leq 2\sum_{t=1}^T\sum_{h=1}^H\left[\bar\beta^t_{h}\left(\epsilon, \frac{\alpha}{2TMH}\right)\left(\sum_{m=1}^M \left\lVert \bphi(z^t_{m, h}) \right\rVert_{(\bLambda^t_{m, h})^{-1}}\right)\right] \\
    &\leq 2\sum_{h=1}^H\left[\bar\beta^T_{h}\left(\epsilon, \frac{\alpha}{2TMH}\right)\left(\sum_{t=1}^T\sum_{m=1}^M \left\lVert \bphi(z^t_{m, h}) \right\rVert_{(\bLambda^t_{m, h})^{-1}}\right)\right]
\end{align*}
Here, the last inequality follows from $\beta^t_h \leq \beta^T_h$ for all $(t, h)\in[T]\times[H]$. To bound variance terms, we use Lemma~\ref{lem:sum_variance_homo}. 
\begin{align*}
    \sum_{t=1}^T\sum_{h=1}^H -\delta^t_h(\bz^t_h) &\leq 2\sum_{h=1}^H\left[\bar\beta^T_{h}\left(\epsilon, \frac{\alpha}{2TMH}\right)\left(\sum_{t=1}^T\sum_{m=1}^M \left\lVert \bphi(z^t_{m, h}) \right\rVert_{(\bLambda^t_{m, h})^{-1}}\right)\right] \\
    &\leq 2\sum_{h=1}^H\left[\bar\beta^T_{h}\left(\epsilon, \frac{\alpha}{2TMH}\right)\left(\sum_{t=1}^T\sum_{m=1}^M \left\lVert \bphi(z^t_{m, h}) \right\rVert_{(\bLambda^t_{m, h})^{-1}}\right)\right]
\end{align*}
We first bound the term $\bar\beta^T_h(\epsilon, \frac{\alpha}{2TMH})$. By Lemma~\ref{lem:homo_beta}, after setting $\epsilon = 3C_bH\sqrt{\log MTH}/T$. Therefore, we have, with probability at least $1-\alpha$, for all $t \in [T], h \in [H]$ and $m \in [M]$ simultaneously,
\begin{align}
    \bar\beta^T_{h}\left(\epsilon, \frac{\alpha}{2TMH}\right) &\leq \sqrt{2}R_Q + 2HC_M\log(TMH)^{1/2}\cdot(\log(MT))^{1/2 + 1/\gamma}\log(2MTH/\alpha)^{1/2}. \\
    &= \cO\left(H\log(TMH)^{\frac{1}{2}}\cdot(\log MT)^{\frac{1}{2} + \tfrac{1}{\gamma}}\log\left(\tfrac{2MTH}{\alpha}\right)^{\tfrac{1}{2}}\right).
\end{align}
Next, for the communication parameter $S$, we have from Lemma~\ref{lem:sum_variance_homo} for each $h \in [H]$ and any $\omega > 1$,
\begin{align}
    \sum_{t=1}^T\sum_{m=1}^M \left\lVert \bphi(z^t_{m, h}) \right\rVert_{(\bLambda^t_{m, h})^{-1}} &\leq  \left(  \frac{2\Gamma_K(MT, \lambda)}{\log \omega} \right)M\sqrt{S} + \omega\sqrt{2MT\Gamma_K(MT, \lambda)}.
\end{align}
By Lemma~\ref{lem:homo_info_gain}, we have that for some fixed absolute constants $C_b$ and sufficiently large $T$,
\begin{align}
    \sum_{t=1}^T\sum_{m=1}^M \left\lVert \bphi(z^t_{m, h}) \right\rVert_{(\bLambda^t_{m, h})^{-1}} &\leq  \left(  \frac{2C_b\log(MT)^{1/\gamma}}{\log \omega} \right)M\sqrt{S} + \omega\sqrt{2MTC_b\log(MT)^{1/\gamma}} \\ \intertext{Setting $\omega = 2$, we have for sufficiently large $T$,}
    &= \cO\left(  \log(MT)^{1/\gamma}M\sqrt{S} + \sqrt{MT\log(MT)^{1/\gamma}}\right).
\end{align}
Putting everything together, we obtain that with probability at least $1-\alpha$,
\begin{align*}
    &\regret(T) = \cO\left(H^2\log(TMH)\cdot(\log MT)^{\frac{1}{2} + \tfrac{1}{\gamma}}\log\left(\tfrac{1}{\alpha}\right)^{\tfrac{1}{2}}\left(\log(MT)^{\frac{1}{\gamma}}M\sqrt{S} + \sqrt{MT\log(MT)^{\frac{1}{\gamma}}} \right)\right) \\
    \implies &\regret(T)=\widetilde\cO\left(H^2\left(M\sqrt{S} + \sqrt{MT}\right)\sqrt{\log\left(\frac{1}{\alpha}\right)}\right).
\end{align*}
\end{proof}

\begin{lemma}[Multi-agent Regret Decomposition in Factored Environments]
For any multi-agent state-action profile $\bz = \{(z_m)_{m \in [M]}\} \in \cZ^M \text{ where, } \cZ = \cS \times \cA,$ define the multi-agent temporal-difference (TD) error $\delta^t_h$ as follows.
\begin{align*}
    \delta^t_h(\bz) = \sum_{m=1}^M \left[r_{m, h}(z_m) + \bbP_{m, h}V^t_{m, h+1}(z_m) - Q^t_{m, h}(z_m)\right].
\end{align*}
Then, for all $(t, h) \in [T]\times[M]$, the group regret decomposes as follows.
\begin{multline*}
    \regret(T) = \sum_{t=1}^T\sum_{h=1}^H \left[ \bbE_{\bpi^\star}\left[ \delta^t_h(\bz) | \x_1 = \x_1^t\right] -\delta^t_h(\bz^t_h)\right] + \sum_{t=1}^T\sum_{h=1}^H\sum_{m=1}^M \left[\xi^1_{t, m, h} + \xi^2_{t, m, h}\right] \\ + \sum_{t=1}^T\sum_{h=1}^H\sum_{m=1}^M \bbE_{\pi^\star_m}\left[\left\langle Q^t_{m, h}(x_m, \cdot), \pi^\star_m(\cdot|x_m) - \pi^t_h(\cdot | x_m)\right\rangle_\cA | \x_1 = \x^t_1\right].
\end{multline*}
\label{lem:regret_decomp_factored}
\end{lemma}
\begin{lemma}[Multi-agent TD-error concentration]
Let $\bz = (z_1, ..., z_M) \in \cZ^M$, $\cZ = \cS \times \cA$ be a multi-agent state-action pair in a parallel environment. For any $t \in [T], h \in [H]$ and $m \in [M]$ we have with probability at least $1-\alpha$,
\begin{equation*}
 \resizebox{0.95\hsize}{!}{%
    $-2\underbrace{\left(\sqrt{d\lambda}+2H\sqrt{\log\left(\frac{\det\left(\lambda\bI_d + \bLambda^t_h\right)}{\det\left(\lambda\bI_d\right)}\right) + Mt(\lambda-1) + 2\log\left(\frac{tM|\cN_\epsilon|}{\alpha}\right) + \frac{2t^2\epsilon^2}{H^2\lambda}}\right)}_{\bar\beta^t_{h}\left(\epsilon, \alpha\right)}\left(\underset{m \in \cM}{\sum}\left\lVert \bphi(z_m) \right\rVert_{(\bLambda^t_{m, h})^{-1}}\right) \leq \delta^t_h(\bz) \leq 0.$
    }
\end{equation*}
\end{lemma}
\begin{proof}
Without loss of generality, assume that the agents are ordered with fixed indices from $1, ..., M$, and let the last global synchronization of state $h \in [H]$ be done after episode $k_t$. Consider therefore the set $\cU^m_h(t) = \left\{ \cup_{\tau=1}^{k_t} \cup_{l=1}^M (x^\tau_{l, h}, a^\tau_{l, h}, x^\tau_{l, h+1}) \right\} \bigcup \left\{ \cup_{\tau=k_t+1}^{t-1}  (x^\tau_{m, h}, a^\tau_{m, h}, x^\tau_{m, h+1}) \right\}$ for all available transitions at step $h$ for agent $m$. After each episode, each agent $m \in [M]$ therefore updates its policy parameters by solving the following ridge regression.
\begin{align}
    \min_{\btheta \in \bbR^d} L(\btheta) = \sum_{(x, a, x') \in \cU^m_h(t)} \left[ r_h(x, a) + V^t_{h+1}(x') - \left\langle \bphi(x, a), \btheta\right\rangle \right]^2 + \lambda \lVert \btheta \rVert_2^2.
\end{align}
As a shorthand, let $U^m_h(t) = \left| \cU^m_h(t) \right|$ denote the size of this observation set, and without loss of generality consider that these observations are ordered as $1, ..., U^m_h(t)$. Consider now the feature matrix $\bPhi^t_{m, h} : \bbR^{U^m_h(t) \times d}$ and covariance $\bLambda^t_{m, h} \in \bbR^{d \times d}$, given as,
\begin{align}
    \bPhi^t_{m, h} :=& \left[ \bphi(x_1, a_1)^\top, \bphi(x_2, a_2)^\top, ..., \bphi(x_{U^m_h(t)}, a_{U^m_h(t)})^\top\right]^\top, \\
    \bLambda^t_{m, h} :=& \sum_{\tau = 1}^{{U^m_h(t)}} \bphi(x_\tau, a_\tau)\bphi(x_\tau, a_\tau)^\top + \lambda \bI_d = \lambda\bI_d + (\bPhi^t_{m, h})^\top(\bPhi^t_{m, h}).
\end{align}
The solution to the above regression problem is given as $\widehat\btheta^t_{m, h} = (\bLambda^t_{m, h})^{-1} \bPhi^t_{m, h}\y^t_{m, h}$, where $\y^t_{m,h}$ is the observation vector, such that $(\y^t_{m, h})_{i} = r_h(x_i, a_i) + V^t_{h+1}(x'_i)$ for $i \in [U^m_h(t)]$. We will also be requiring two additional quantities for the proof, defined as follows. Let $\cU_{h}(t) = \bigcup_{m=1}^M \bigcup_{\tau=1}^{t-1} \left\{\left(x^t_{m, h}, a^t_{m, h}, x^t_{m, h+1}\right)\right\}$ and $\left|\cU_h(t)\right| = M(t-1)$, and $\left\{\left(x_\tau, a_\tau, x'_\tau\right) \right\}_{\tau=1}^{M(t-1)}$ be an ordering of $\cU_h(t)$. Then, we define the \textit{global} covariance matrix as,
\begin{align}
    \bPhi^t_h &= \left[ \bphi(x_1, a_1)^\top, \bphi(x_2, a_2)^\top, ..., \bphi(x_{M(t-1)}, a_{M(t-1)})^\top\right]^\top\\
    \bLambda^t_h &= (\bPhi^t_h)^\top\bPhi^t_h.
\end{align}
We will be bounding the overall temporal-difference error function $\delta^t_h = \sum_{m=1}^M \delta^t_{m, h}$ in terms of the \textit{global} quantity described above. For any agent $m$, the temporal difference error in state $h$ of episode $t$ is given as,
\begin{align}
    \delta_{m, h}^t(x, a) = r_h(x, a) + \bbP_h V^t_{m, h+1} - Q^t_{m, h}(x, a) = \bbT^\star_h Q^t_{m, h+1} - Q^t_{m, h},
\end{align}
Where $\bbT^\star_h$ is the Bellman optimality operator. By Definition~\ref{def:linear_mdp} there exists a parameter $\bar\btheta^t_{m, h}$ such that $\bbT^\star_hQ^t_{m, h+1}(z) = \bphi(z)^\top\bar\btheta^t_{m, h}$ and $\lVert \bar\btheta^t_{m, h} \rVert \leq 2H\sqrt{d}$. Consider now the difference between the estimated Bellman operator $\bphi(z)^\top\widehat\btheta^t_{m, h}$ and the true Bellman operator $\bphi(z)^\top\bar\btheta^t_{m, h}$. We have, for any $z \in \cZ$,
\begin{align*}
    &\bphi(z)^\top\widehat\btheta^t_{m, h} - \bphi(z)^\top\bar\btheta^t_{m, h} \\
    &= \bphi(z)^\top(\bLambda^t_{m, h})^{-1}(\bPhi^t_{m, h})^\top\left(\y^t_{m, h} - \bPhi^t_{m, h}\bar\btheta^t_{m, h}\right) - \lambda\cdot \bphi(z)^\top(\bLambda_{m, h}^t)^{-1}\bar\btheta^t_{m, h} \\
    &\leq \underbrace{\left| \bphi(z)^\top(\bLambda^t_{m, h})^{-1}(\bPhi^t_{m, h})^\top\left(\y^t_{m, h} - \bPhi^t_{m, h}\bar\btheta^t_{m, h}\right) \right|}_{\text{(A)}} + \underbrace{\left|\lambda\cdot \bphi(z)^\top(\bLambda_{m, h}^t)^{-1}\bar\btheta^t_{m, h}\right|}_{\text{(B)}}
\end{align*}
We first bound term (B). By Cauchy-Schwarz, we have,
\begin{align*}
    \left|\lambda\cdot \bphi(z)^\top(\bLambda_{m, h}^t)^{-1}\bar\btheta^t_{m, h}\right| &\leq \left\lVert \lambda (\bLambda_{m,h}^t)^{-1}\bphi(z) \right\rVert_2\cdot \left\lVert \bar\btheta^t_{m, h} \right\rVert_2 \leq 2H\sqrt{d} \left\lVert \lambda (\bLambda_{m,h}^t)^{-1}\bphi(z) \right\rVert_2 \\
    &\leq 2H\sqrt{d\lambda}\left\lVert \bphi(z) \right\rVert_{(\bLambda^t_{m, h})^{-1}}
\end{align*}
The second inequality above follows from the fact that $\lVert \bar\btheta^t_{m, h} \rVert_2 \leq 2H\sqrt{d}$. The third inequality follows from the fact that $\bLambda^t_{m, h} \succcurlyeq \lambda\bI_d$. Now let us bound term (A). Let the previous synchronization step be given by $k_t < t$. Therefore, any agent $m$ at time $t$ has a total of $t_{m, h} = Mk_t + (t-k_t)$ records for step $h \in [H]$. Without loss of generality, consider a permutation $\bmu$ of $[t_{m, h}]$ that maps the first $Mk_t$ elements as follows. The agent-episode pair $(n, l)$ maps to the index $i = M\cdot(l-1) + n$, and $i \in [Mk_t]$. The last $(t-k_t)$ entries of $\bmu$ refer to the observations from agent $m$ for episodes $k_t +1, ..., t$. Therefore, for each $(l, n)$ in $[M \times k_t]$ there exists a corresponding $i \in \bmu$ such that $i \leq Mk_t$ and
\begin{align}
    [\y^t_{m, t}]_i - [\Phi^t_{m, h}\bar\btheta_{m, h}]_i &= r_h(x^l_{n, h}, a^l_{n, h}) + V^t_{m, h+1}(x^l_{n, h+1}) - \bphi(x^l_{n, h}, a^l_{n, h})^\top \bar\btheta^t_{m, h} \\
    &= r_h(x^l_{n, h}, a^l_{n, h}) + V^t_{m, h+1}(x^l_{n, h+1}) - \bbT^\star_hQ^t_{m, h+1}(x^l_{n, h}, a^l_{n, h}) \\
    &= V^t_{m, h+1}(x^l_{n, h+1}) - (\bbP_h V^t_{m, h+1})(x^l_{n, h}, a^l_{n, h})
\end{align}
Furthermore, for any  $l \in [k_t + 1, t - 1]$ there exists an $i \in \bmu$ such that $i > Mk_t$ and,
\begin{align}
    [\y^t_{m, t}]_i - [\Phi^t_{m, h}\bar\btheta_{m, h}]_i &= r_h(x^l_{m, h}, a^l_{m, h}) + V^t_{m, h+1}(x^l_{m, h+1}) - \bphi(x^l_{m, h}, a^l_{m, h})^\top \bar\btheta^t_{m, h} \\
    &= r_h(x^l_{m, h}, a^l_{m, h}) + V^t_{m, h+1}(x^l_{m, h+1}) - \bbT^\star_hQ^t_{m, h+1}(x^l_{m, h}, a^l_{m, h}) \\
    &= V^t_{m, h+1}(x^l_{m, h+1}) - (\bbP_h V^t_{m, h+1})(x^l_{m, h}, a^l_{m, h})
\end{align}
For brevity, consider the replacement:
\begin{multline}
    \bS^t_{m, h} = \sum_{n=1}^M \sum_{\tau=1}^{k_t}\bphi(x^\tau_{n, h}, a^\tau_{n, h}) \left[V^t_{m, h+1}(x^\tau_{n, h+1})- (\bbP_hV^t_{m, h+1})(x^\tau_{n, h}, a^\tau_{n, h})\right] \\+ \sum_{\tau = k_t + 1}^{t-1} \bphi(x^\tau_{m, h}, a^\tau_{m, h})\left[V^t_{m, h+1}(x^\tau_{m, h+1})- (\bbP_hV^t_{m, h+1})(x^\tau_{m, h}, a^\tau_{m, h})\right]
\end{multline}
Replacing the above decomposition we obtain, for any $z \in \cZ$, for term (A),
\begin{align}
    \left| \bphi(z)^\top(\bLambda^t_{m, h})^{-1}(\bPhi^t_{m, h})^\top\left(\y^t_{m, h} - \bPhi^t_{m, h}\bar\btheta^t_{m, h}\right) \right| &= \left| \bphi(z)^\top (\bLambda^t_{m, h})^{-1}\bS^t_{m, h}\right| \\
    &\leq \left\lVert \bphi(z) \right\rVert_{(\bLambda^t_{m, h})^{-1}}\cdot \left\lVert \bS^t_{m, h} \right\rVert_{(\bLambda^t_{m, h})^{-1}}.
\end{align}
We will bound the term $ \left\lVert \bS^t_{m, h} \right\rVert_{(\bLambda^t_{m, h})^{-1}}$ by a self-normalized stochastic process concentration, and a union bound over a covering of the appropriate function class, as done in the single-agent analysis for~\cite{yang2020provably}. There are several key differences, however, compared to the single-agent analysis. Lemma~\ref{lem:beta_independent_centralized} provides the required bound. Now, for each $m \in [M], t \in [T]$ and $h \in [H]$ we have that $\log\det\left( \bLambda^t_{m, h}\right) \leq \log\det\left(\bLambda^t_{h}\right)$.
Next, we set 
\begin{align*}
    \beta^t_{m, h}(\epsilon, \delta') = 2H\sqrt{d\lambda}+2H\sqrt{\log\left(\frac{\det\left(\bLambda^t_{m,h}\right)}{\det\left(\lambda\bI_d\right)}\right) +Mt(\lambda-1) + 2\log\left(\frac{t\cdot|\cN_\epsilon|}{\delta'}\right) + \frac{2M^2t^2\epsilon^2}{H^2\lambda}},
\end{align*}
and $\bar\beta^t_{h}(\epsilon, \delta') = 2H\sqrt{d\lambda}+\sqrt{ 4H^2\cdot\log\left(\frac{\det\left(\bLambda^t_{h}\right)}{\det\left(\lambda\bI_d\right)}\right) + 4H^2Mt\lambda + 8H^2\log\left(\frac{t\cdot|\cN_\epsilon|}{\delta'}\right) + \frac{8M^2t^2\epsilon^2}{\lambda}}$. With this substitution, and a union bound, we can say that with probability at least $1-\delta'$, for any $\bz = (z_1, ..., z_M) \in \cZ^M$, we have,
\begin{align*}
    \delta^t_h(\bz) = \sum_{m=1}^M \delta^t_{m, h}(z_m) &= \sum_{m=1}^M \bphi(z_m)^\top\widehat\btheta^t_{m, h} - \bphi(z_m)^\top\bar\btheta^t_{m, h} \\
    &\leq \sum_{m=1}^M \left( \left\lVert \bphi(z_m) \right\rVert_{(\bLambda^t_{m, h})^{-1}}\left(\sqrt{d\lambda} + \left\lVert \bS^t_{m, h} \right\rVert_{(\bLambda^t_{m, h})^{-1}}\right) \right)\\
    &\leq \sum_{m=1}^M \left( \beta^t_{m, h}(\epsilon, \delta'/M)\left\lVert \bphi(z_m) \right\rVert_{(\bLambda^t_{m, h})^{-1}}\right) \\
    &\leq \bar\beta^t_{h}(\epsilon, \delta'/M)\left(\sum_{m=1}^M \left\lVert \bphi(z_m) \right\rVert_{(\bLambda^t_{m, h})^{-1}}\right).
\end{align*}
Here, the first equality follows from the independence of the environments, and the second inequality follows by first applying Lemma~\ref{lem:beta_independent_centralized} with probability $\delta'/M$ to each of the $M$ terms, and then applying a union bound over all the agents. Finally, we obtain the final form of the proof by the following decomposition.
\begin{align*}
    -\delta^t_h(\bz) &= \sum_{m=1}^M \left[Q^t_{m, h}(z_m) - \bphi(z_m)^\top\bar\btheta^t_{m, h}\right] \\
    &\leq \sum_{m=1}^M \bphi(z_m)^\top\left[ \widehat\btheta^t_{m, h} - \bar\btheta^t_{m, h}\right] + \bar\beta^t_{h}\left(\epsilon, \frac{\alpha'}{M}\right)\left(\sum_{m=1}^M \left\lVert \bphi(z_m) \right\rVert_{(\bLambda^t_{m, h})^{-1}}\right) \\
    &\leq 2\bar\beta^t_{h}\left(\epsilon, \frac{\alpha'}{M}\right)\left(\sum_{m=1}^M \left\lVert \bphi(z_m) \right\rVert_{(\bLambda^t_{m, h})^{-1}}\right).
\end{align*}
Here, the first inequality is true from the greedy UCB policy of the algorithm, and the second inequality holds with probability at least $1-\alpha'$.
\end{proof}

\begin{lemma}[Variance control via communication in homogenous factored environments]
\label{lem:sum_variance_homo}
Let Algorithm~\ref{alg:ind_homo} be run for any $T > 0$ and $M \geq 1$, with $S$ as the communication control factor. Then, the following holds for the cumulative variance.
\begin{align}
    \sum_{m=1}^M\sum_{t=1}^T \left\lVert \bphi(z^t_{m, h}) \right\rVert_{(\bLambda^t_{m, h})^{-1}} \leq  2\log\left(\frac{\det\left( \bLambda^T_h\right)}{\det\left(\lambda\bI_d\right)}\right)\left(\frac{M}{\log 2}\right)\sqrt{S} + 2\sqrt{2MT\log\left(\frac{\det\left( \bLambda^T_h\right)}{\det\left(\lambda\bI_d\right)}\right)}.
\end{align}
\end{lemma}
\begin{proof}
Consider the following mappings $\nu_M, \nu_T : [MT] \rightarrow [M] \times [T]$.
\begin{align}
    \nu_M(\tau) = \tau (\text{mod } M), \text{and } \nu_T = \left\lceil \frac{\tau}{M}\right\rceil.
\end{align}
Now, consider $\bar\bLambda^\tau_h = \lambda\bI_d + \sum_{u=1}^\tau \bphi\left(z^{\nu_T(u)}_{\nu_M(u), h}\right)\bphi\left(z^{\nu_T(u)}_{\nu_M(u), h}\right)^\top$ for $\tau > 0$ and $\bar\bLambda^0_h = \lambda\bI_d$. Furthermore, assume that global synchronizations occur at round $\bsigma = (\sigma_{1}, ..., \sigma_{n})$ where there are a total of $n-1$ rounds of synchronization and $\sigma_{i} \in [T] \forall\ i \in [N-1]$ and $\sigma_{n} = T$, i.e., the final round.
Let $R_h = \left\lceil  \log\left(\frac{\det\left(\bar\bLambda^T_{h}\right)}{\det\left(\lambda\bI_d\right)}\right) \right\rceil$. It follows that there exist at most $R_h$ periods between synchronization (i.e., intervals $\sigma_{k-1}$ to $\sigma_k$ for $k \in [N]$) in which the following does not hold true:
\begin{align}
    \label{eqn:interval_sync_single_agent}
    1 \leq \frac{\det(\bar\bLambda^{\sigma_{k}}_h)}{\det(\bar\bLambda^{k-1}_h)}\leq 2.
\end{align}
Let us denote the event when Equation~(\ref{eqn:interval_sync_single_agent}) does holds for an interval $\sigma_{k-1}$ to $\sigma_{k}$ as $E$. Now, for any $t \in [\sigma_{k-1}, \sigma_{k}]$, we have, for any $m \in [M]$,
\begin{align}
    \left\lVert \bphi(z^t_{m, h}) \right\rVert_{(\bLambda^t_{m, h})^{-1}} &\leq \left\lVert \bphi(z^t_{m, h}) \right\rVert_{(\bar\bLambda^{t}_{h})^{-1}}\sqrt{\frac{\det\left(\bar\bLambda^t_{h}\right)}{\det\left(\bLambda^t_{m,h}\right)}} \leq \left\lVert \bphi(z^t_{m, h}) \right\rVert_{(\bar\bLambda^t_{h})^{-1}}\sqrt{\frac{\det\left(\bar\bLambda^{\sigma_{k}}_{ h}\right)}{\det\left(\bar\bLambda^{\sigma_{k-1}}_{h}\right)}} \leq 2\left\lVert \bphi(z^t_{m, h}) \right\rVert_{(\bar\bLambda^{t}_{h})^{-1}}.
\end{align}
Here, the first inequality follows from the fact that $\bLambda^t_{m, h} \preccurlyeq \bar\bLambda^t_{h}$, the second inequality follows from the fact that $\bLambda^t_{m, h} \preccurlyeq \bar\bLambda^{\sigma_{k}}_{h} \implies \det(\bLambda^t_{m, h}) \leqslant \det(\bar\bLambda^{\sigma_{k}}_{h})$, and $\bLambda^t_{m, h} \succcurlyeq \bar\bLambda^{\sigma_{k-1}}_{h} \implies \det(\bLambda^t_{m, h}) \geqslant \det(\bar\bLambda^{\sigma_{k-1}}_{h})$; and the final inequality follows from the fact that event $E$ holds. Now, we can consider the partial sums only in the intervals for which event $E$ holds. For any $t \in [T]$, consider $\sigma(t) = \max_{i \in [N]} \{\sigma_{i} | \sigma_{i} \leq t\}$ denote the last round of synchronization prior to episode $t$. Then,
\begin{align}
    \sum_{t: E\text{ is true}}^T\sum_{m=1}^M \left\lVert \bphi(z^t_{m, h}) \right\rVert_{(\bLambda^t_{m, h})^{-1}} &\leq \sqrt{MT\sum_{m=1}^M\sum_{t: E\text{ is true}}^T \left\lVert \bphi(z^t_{m, h}) \right\rVert^2_{(\bLambda^t_{m, h})^{-1}}} \\
    &\leq 2\sqrt{MT\sum_{m=1}^M\sum_{t: E\text{ is true}}^T \left\lVert \bphi(z^t_{m, h}) \right\rVert^2_{(\bar\bLambda^t_{h})^{-1}}}\\
    &\leq 2\sqrt{MT\sum_{m=1}^M\sum_{t=1}^T \left\lVert \bphi(z^t_{m, h}) \right\rVert^2_{(\bar\bLambda^t_{h})^{-1}}}\\
    &=2\sqrt{MT\sum_{m=1}^M\sum_{\tau=1}^T \left\lVert \bphi(z^{\nu_T(\tau)}_{\nu_M(\tau), h}) \right\rVert^2_{(\bar\bLambda^t_{h})^{-1}}} \\
    &= 2\sqrt{MT\log\left(\frac{\det\left( \bLambda^T_h\right)}{\det\left(\lambda\bI_d\right)}\right)}.
\end{align}
Here, the first inequality follows from Cauchy-Schwarz, the second inequality follows from the fact that event $E$ holds, and the final equality follows from Lemma~\ref{lem:variance_sum}. Now, we sum up the cumulative sum for episodes when $E$ does not hold. Consider an interval $\sigma_{k-1}$ to $\sigma_{k}$ for $k \in [N]$ of length $\Delta_{k} = \sigma_{k} - \sigma_{k-1}$ in which $E$ does not hold. We have that,
\begin{align}
    \sum_{m=1}^M\sum_{t=\sigma_{k-1}}^{\sigma_k} \left\lVert \bphi(z^t_{m, h}) \right\rVert_{(\bLambda^t_{m, h})^{-1}} &\leq \sum_{m=1}^M\sqrt{\Delta_{k, h}\sum_{t=\sigma_{k-1}}^{\sigma_k} \left\lVert \bphi(z^t_{m, h}) \right\rVert^2_{(\bLambda^t_{m, h})^{-1}}} \\
    &\leq \sum_{m=1}^M\sqrt{\Delta_{k, h}\cdot \log_\omega\left(\frac{\det(\bLambda^{\sigma_{k}}_{m, h})}{\det(\bLambda^{\sigma_{k-1}}_{m, h})}\right)} \\
    &\leq \sum_{m=1}^M\sqrt{\Delta_{k, h}\cdot \log_\omega\left(\frac{\det(\bar\bLambda^{\sigma_k}_{ h})}{\det(\bar\bLambda^{\sigma_{k-1}}_{ h})}\right)} \\
    &\leq M\sqrt{S}.
\end{align}
The last inequality follows from the synchronization criterion. Now, note that there are at most $R_h$ periods in which event $E$ does not hold, and hence the total sum in this period can be bound as,
\begin{align}
    \sum_{(t : E \text{ is not true})}^T \sum_{m=1}^M\left\lVert \bphi(z^t_{m, h}) \right\rVert_{(\bLambda^t_{m, h})^{-1}} &\leq R_hM\sqrt{S} \leq \left(  \log\left(\frac{\det\left( \bLambda^T_h\right)}{\det\left(\lambda\bI_d\right)}\right)+ 1\right)M\sqrt{S}.
\end{align}
Therefore, we can bound the total variance as,
\begin{align*}
    \sum_{m=1}^M\sum_{t=1}^T \left\lVert \bphi(z^t_{m, h}) \right\rVert_{(\bLambda^t_{m, h})^{-1}} &\leq  \left(  \log\left(\frac{\det\left( \bLambda^T_h\right)}{\det\left(\lambda\bI_d\right)}\right) + 1\right)M\sqrt{S} + 2\sqrt{MT\log\left(\frac{\det\left( \bLambda^T_h\right)}{\det\left(\lambda\bI_d\right)}\right)} \\
    &\leq  2\log\left(\frac{\det\left( \bLambda^T_h\right)}{\det\left(\lambda\bI_d\right)}\right)\left(\frac{M}{\log 2}\right)\sqrt{S} + 2\sqrt{2MT\log\left(\frac{\det\left( \bLambda^T_h\right)}{\det\left(\lambda\bI_d\right)}\right)}.
\end{align*}
\end{proof}
\begin{lemma}[$\beta$-concentration for homogenous independent environments]
For sufficiently large $T$, $\lambda = 1 + 1/MT$ and $\epsilon^* = 3C_bH\sqrt{\log MTH}/T$ for a sufficiently large constant $C, C'$, we have that for any $h \in [H], M > 1, T > 1$ with probability at least $1-\delta'$,
\begin{align*}
     \beta^*_h(\delta) = \leq H\sqrt{d\lambda}+2H\sqrt{(d+2)\log\frac{t+\lambda}{\lambda} + 2\log\left(\frac{1}{\alpha}\right) + C'd^2 \log\left(1 + 8Cd^{1/2}T^2\log(TMH)\right) + 3}.
\end{align*}
Where $C_M$ is an absolute constant independent of $T, M$ and $H$.
\label{lem:homo_beta}
\end{lemma}
\begin{proof}
Recall that $\bar\beta^t_{h}(\epsilon, \delta') =H\sqrt{d\lambda}+2H\sqrt{\log\left(\frac{\det\left( \bLambda^t_h\right)}{\det\left(\lambda\bI_d\right)}\right) + Mt(\lambda-1) + 2\log\left(\frac{t|\cN_\epsilon|}{\alpha}\right) + \frac{2t^2\epsilon^2}{H^2\lambda}}$. By setting $\lambda = 1 + 1/(MT)$, we have that
\begin{align}
    \bar\beta^t_{h}(\epsilon, \delta') &= H\sqrt{d\lambda}+2H\sqrt{\log\left(\frac{\det\left( \bLambda^t_h\right)}{\det\left(\lambda\bI_d\right)}\right) + Mt(\lambda-1) + 2\log\left(\frac{t|\cN_\epsilon|}{\alpha}\right) + \frac{2t^2\epsilon^2}{H^2\lambda}}\\
    &=H\sqrt{d\lambda}+2H\sqrt{\log\left(\frac{\det\left( \bLambda^t_h\right)}{\det\left(\lambda\bI_d\right)}\right) + \frac{t}{T} + 2\log\left(\frac{t|\cN_\epsilon|}{\alpha}\right) + \frac{2t^2\epsilon^2}{H^2\lambda}}\tag{since $\lambda = 1 + (HMT)^{-1}$}\\
    &=H\sqrt{d\lambda}+2H\sqrt{d\log\frac{t+\lambda}{\lambda} + \frac{t}{T} + 2\log\left(\frac{t|\cN_\epsilon|}{\alpha}\right) + \frac{2t^2\epsilon^2}{H^2\lambda}}\tag{AM $\geqslant$ GM followed by determinant-trace inequality}
\end{align}
Here $\cN_\epsilon$ is an $\epsilon-$covering of the function class $\cV_{\text{UCB}}$ for any $h \in [H], m \in [M]$ or $t \in [T]$ under the distance function $\text{dist}(V, V') = \sup_{x \in \cS} |V(x) - V'(x)|$. To bound this quantity by the appropriate covering number, we first observe that for any $V \in \cV_{\text{UCB}}$, we have that the policy weights are bounded as $2H\sqrt{dMT/\lambda}$ (Lemma~\ref{lem:weight_norm_homo_value}). Therefore, by Lemma~\ref{lem:covering_ind_homo} we have for any constant $B$ such that $\beta^t_{m, h} \leq B$,
\begin{align}
    \log \cN_\varepsilon \leq d \log\left(1+8H\sqrt{\frac{dMT}{\lambda\epsilon^2}}\right) + d^2 \log\left(1 + \frac{8d^{1/2}B^2}{\lambda\epsilon^2}\right).
\end{align}
Recall that we select the hyperparameters $\lambda = 1-(HMT)^{-1}$ and $\beta = \cO(dH\sqrt{\log(TMH)}$, and to balance the terms in $\bar\beta^t_h$ we select $\epsilon = \epsilon^\star = dH/T$. Finally, we obtain that for some absolute constant $C$, by replacing the above values,
\begin{align}
    \log \cN_\varepsilon \leq d \log\left(1+8\sqrt{\frac{MT^3}{d}}\right) + d^2 \log\left(1 + 8Cd^{1/2}T^2\log(TMH)\right).
\end{align}
Therefore, for some absolute constant $C'$ independent of $M, T, H, d$ and $C$, we have,
\begin{align}
    \log \cN_\varepsilon \leq C'd^2 \log\left(CdT\log(TMH)\right).
\end{align}
Replacing this result in $\bar\beta^t_h$ we have that,
\begin{align}
    \bar\beta^t_{h}(\epsilon, \delta') &\leq H\sqrt{d\lambda}+2H\sqrt{(d+2)\log\frac{t+\lambda}{\lambda} + 2\log\left(\frac{1}{\alpha}\right) + C'd^2 \log\left(1 + 8Cd^{1/2}T^2\log(TMH)\right) + 3}.
\end{align}
\end{proof}
\begin{lemma}
\label{lem:beta_independent_centralized}
For any $m \in [M], h \in [H]$ and $t \in [T]$, let $k_t$ denote the episode after which the last global synchronization has taken place, and $\bS^t_{m, h}$ and $\bLambda^k_t$ be defined as follows.
\begin{multline*}
    \bS^t_{m, h} = \sum_{n=1}^M \sum_{\tau=1}^{k_t}\bphi(x^\tau_{n, h}, a^\tau_{n, h}) \left[V^t_{m, h+1}(x^\tau_{n, h+1})- (\bbP_hV^t_{m, h+1})(x^\tau_{n, h}, a^\tau_{n, h})\right] \\+ \sum_{\tau = k_t + 1}^{t-1} \bphi(x^\tau_{m, h}, a^\tau_{m, h})\left[V^t_{m, h+1}(x^\tau_{m, h+1})- (\bbP_hV^t_{m, h+1})(x^\tau_{m, h}, a^\tau_{m, h})\right],
\end{multline*} 
\begin{align*}
    \bLambda^t_{m, h} =  \sum_{n=1}^M \sum_{\tau=1}^{k_t}\bphi(x^\tau_{n, h}, a^\tau_{n, h})\bphi(x^\tau_{n, h}, a^\tau_{n, h})^\top + \sum_{\tau = k_t + 1}^{t-1} \bphi(x^\tau_{m, h}, a^\tau_{m, h})\bphi(x^\tau_{m, h}, a^\tau_{m, h})^\top + \lambda\bI_d.
\end{align*}
Where $V \in \cV$ and $\cN_\epsilon$ denotes the $\epsilon-$covering of the value function space $\cV$. Then, with probability at least $1-\delta$,
\begin{align*}
    \sup_{k_t \leq t, V \in \cV}\left\lVert \bS^t_{m, h} \right\rVert_{(\bLambda^t_{m, h})^{-1}} &\leq 2H\sqrt{ \log\left(\frac{\det\left(\bLambda^t_{m,h}\right)}{\det\left(\lambda\bI_d\right)}\right) + Mt(\lambda-1) + 2\log\left(\frac{t\cdot|\cN_\epsilon|}{\delta}\right) + \frac{2M^2t^2\epsilon^2}{H^2\lambda}}.
\end{align*}
\end{lemma}
\begin{proof}
Note that for any agent $m$, the function $V^t_{m, h+1}$ depends on the historical data from all $M$ agents from the first $k_t$ episodes, and the personal historical data for the first $(t-1)$ episodes, and depends on
\begin{align}
    \cU^m_h(t) = \left(\cup_{n \in [M], \tau \in [k_t]}\{(x^\tau_{n, h}, a^\tau_{n, h}, x^\tau_{n, h+1})\}\right) \bigcup \left(\cup_{\tau \in [k_t+1, t-1} \{(x^\tau_{m, h}, a^\tau_{m, h}, x^\tau_{m, h+1})\}\right).
\end{align}

To bound the term we will construct an appropriate filtration to use a self-normalized concentration defined on elements of $\cU^m_h(t)$. We highlight that in the multi-agent case with stochastic communication, it is not straightforward to provide a uniform martingale concentration that holds for all $t \in [T]$ simultaneously (as is done in the single-agent case), as the stochasticity in the environment dictates when communication will take place, and subsequently the quantity considered within self-normalization will depend on this communication itself. To circumvent this issue, we will first fix $k_t \leq t$ and obtain a filtration for a fixed $k_t$. Then, we will take a union bound over all $k_t \in [t]$ to provide the final self-normalized bound. We first fix $k_t$ as a constant quantity known \textit{a priori}, and define the following mappings where $i \in \left[M(t-1)\right], l \in [t-1], $ and $n \in [M]$.
\begin{align*}
    \mu(i) = \left\lceil \frac{i}{M} \right\rceil,
    \nu(i) = i (\text{mod } M), \text{ and, }
    \eta(l, n) = l\cdot(M+1) + n - 1.
\end{align*}  
Now, for a fixed $k_t$, consider the stochastic processes $\{\tilde x_\tau\}_{\tau = 1}^\infty$ and $\{\tilde\bphi_\tau\}_{\tau = 1}^\infty$, where,
\begin{align*}
   \tilde \bphi_i = \bphi(x^{\nu(i)}_{\mu(i), h+1}) \otimes \bone_d\left\{ \left(\mu(i) = m\right) \lor \left(\nu(i) \leq k_t\right)\right\}
\end{align*} 
Here $\otimes$ denotes the Hadamard product, and $\bone_{d}$ is the indicator function in $\bbR^d$. Consider now the filtration $\{\cF_\tau\}_{\tau=0}^\infty$, where $\cF_0$ is empty, and $\cF_\tau = \sigma\left(\left\{ \bigcup (\tilde x_i, \tilde \bphi_i)\right\}_{i \leq \tau}\right)$, where $\sigma(\cdot)$ denotes the corresponding $\sigma-$algebra formed by the set.

At any instant $t$ for any agent $m$, the function $V^t_{m, h+1}$ and features $\bphi(x^t_{m, h}, a^t_{m, h})$ depend only on historical data from all other agents $[M] \setminus \{m\}$ up to the last episode of synchronization $k_t \leq t - 1$ and depend on the personal data up to episode $t-1$. Hence, both are $V^t_{m, h+1}$ and $\bphi(x^t_{m, h}, a^t_{m, h})$ are measurable with respect to 
\begin{align*}
    \sigma\left(\left\{ \bigcup_{l=1}^{k_t}\bigcup_{n=1}^{M} (\tilde x_{\eta(l, n)}, \tilde \bphi_{\eta(l, n)})\right\} \bigcup \left\{\bigcup_{l=k_t+1}^{t-1} (\tilde x_{\eta(l, m)}, \tilde\bphi_{\eta(l, m)})\right\} \right).
\end{align*}
This is a subset of $\cF_{\eta(t, m)}$. Therefore $V^t_{m, h+1}$ is $\cF_{\eta(t, m)}-$measurable for fixed $k_t$. Now, consider $\cU^m_h(\tau)$, the set of features available to agent $m$ at episode $\tau \leq t$. We therefore have that, for any value function $V$,
\begin{align*}
    &\sum_{\tau=1}^{M(t-1)} \btphi_{m, h}(\tau)\left\{ V(\tilde x_\tau) - \bbE[V(\tilde x_\tau) | \cF_{\tau-1}] \right\} \\
    &= \sum_{\tau=1}^{M(t-1)} \left[ \bphi(x^{\nu(i)}_{\mu(i), h+1}) \otimes \bone_d\left\{ \left(\mu(i) = m\right) \lor \left(\nu(i) \leq k_t\right)\right\}\right]\left\{ V(\tilde x_\tau) - \bbE\left[V(\tilde x_\tau) | \cF_{\tau-1}\right] \right\} \\
    &= \sum_{(x_\tau, a_\tau, x'_\tau) \in \cU^m_h(t)} \bphi(x_\tau, a_\tau)\left\{ V(x'_\tau) - \bbE[V(x'_\tau) | \cF_{\tau-1}] \right\}. 
\end{align*}
Now, when $V = V^t_{m, h+1}$, we have from the above,
\begin{align*}
    \sum_{\tau=1}^{M(t-1)} \btphi_\tau\left\{ V^t_{h, m+1}(\tilde x_\tau) - \bbE[V^t_{h, m+1}(\tilde x_\tau) | \cF_{\tau-1}]\right\} = \sum_{(x_\tau, a_\tau, x'_\tau) \in \cU^m_h(t)} \bphi(x_\tau, a_\tau)\left\{ V^t_{m, h+1}(x'_\tau) - \bbE[V^t_{m, h+1}(x'_\tau) | \cF_{\tau-1}] \right\} = \bS^t_{m, h}. 
\end{align*}
Furthermore, consider $\widetilde\bLambda^t_{m, h} = \lambda \bI_d + \sum_{\tau=1}^{M(t-1)} \btphi_\tau\btphi_\tau^\top$. For the second term, we have,
\begin{align*}
     &\widetilde\bLambda^t_{m, h}=\lambda \bI_d +\sum_{\tau=1}^{M(t-1)} \btphi_\tau\btphi_\tau^\top \\
     =&\lambda \bI_d + \sum_{\tau=1}^{M(t-1)} \left[\bphi(x^{\nu(i)}_{\mu(i), h+1}) \otimes \bone_d\left\{ \left(\mu(i) = m\right) \lor \left(\nu(i) \leq k_t\right)\right\}\right]\left[\bphi(x^{\nu(i)}_{\mu(i), h+1}) \otimes \bone_d\left\{ \left(\mu(i) = m\right) \lor \left(\nu(i) \leq k_t\right)\right\}\right]^\top \\
     =&\lambda \bI_d +\sum_{(x_\tau, a_\tau, x'_\tau) \in\cU^m_h(t)} \bphi(x_\tau, a_\tau)\bphi(x_\tau, a_\tau)^\top = \bLambda^t_{m, h}.
\end{align*}
To complete the proof, we bound $\left\lVert \sum_{\tau=1}^{M(t-1)} \widetilde\bphi_{m, h}(\tau)\left\{V^t_{h, m+1}(\tilde x_\tau) - \bbE[V^t_{h, m+1}(\tilde x_\tau) | \cF_{\tau-1}]\right\} \right\rVert_{(\widetilde\bLambda^t_{m, h})^{-1}}$ over all $k_t \in [t]$. We proceed following a self-normalized martingale bound and a covering argument, as done in~\cite{yang2020provably}.

Applying Lemma~\ref{lem:self_normalized_single_task} to  $\left\lVert \sum_{\tau=1}^{M(t-1)} \widetilde\bphi_{m, h}(\tau)\left\{V^t_{h, m+1}(\tilde x_\tau) - \bbE[V^t_{h, m+1}(\tilde x_\tau) | \cF_{\tau-1}]\right\} \right\rVert_{(\widetilde\bLambda^t_{m, h})^{-1}}$ under the filtration $\{\cF_\tau\}_{\tau=0}^\infty$ described earlier, we have that with probability at least $1-\delta'$,
\begin{align*}
    \left\lVert \bS^t_{m, h} \right\rVert^2_{(\bLambda^t_{m, h})^{-1}} &= \left\lVert \sum_{\tau=1}^{M(t-1)} \btphi_\tau\left\{V^t_{h, m+1}(\tilde x_\tau) - \bbE[V^t_{h, m+1}(\tilde x_\tau) | \cF_{\tau-1}]\right\} \right\rVert^2_{(\widetilde\bLambda^t_{m, h})^{-1}} \\
    &\leq \sup_{V \in \cV} \left\lVert \sum_{\tau=1}^{M(t-1)} \btphi_\tau\left\{V(\tilde x_\tau) - \bbE[V(\tilde x_\tau) | \cF_{\tau-1}]\right\} \right\rVert^2_{(\widetilde\bLambda^t_{m, h})^{-1}} \\
    &\leq 4H^2\cdot\log\frac{\det\left(\widetilde\bLambda^t_{m,h}\right)}{\det\left(\lambda\bI_d\right)} + 4H^2Mt(\lambda-1) + 8H^2\log(|\cN_\epsilon|/\delta') + 8M^2t^2\epsilon^2/\lambda.
\end{align*}
Where $\cN_\epsilon$ is an $\epsilon-$covering of $\cV$. Therefore, we have that, with probability at least $1-\delta'$, for any fixed $k_t \leq t$,
\begin{align*}
    \left\lVert \bS^t_{m, h} \right\rVert_{(\bLambda^t_{m, h})^{-1}} &\leq 2H\sqrt{ \log\left(\frac{\det\left(\widetilde\bLambda^t_{m,h}\right)}{\det\left(\lambda\bI_d\right)}\right) + Mt(\lambda-1) + 2\log\left(\frac{|\cN_\epsilon|}{\delta}\right) + \frac{2M^2t^2\epsilon^2}{H^2\lambda}}.
\end{align*}
Taking a union bound over all $k_t \in [t]$ and replacing $\delta' = \delta/t$ gives us the final result.
\end{proof}

\subsection{Cumulative Regret in Heterogenous Independent Environments}
\begin{lemma}[Multi-agent TD-error concentration]
Let $\bz = (z_1, ..., z_M) \in \cZ^M$, $\cZ = \cS \times \cA$ be a multi-agent state-action pair in a factored, independent environment. For any $t \in [T], h \in [H]$ and $m \in [M]$ fix   $\beta^t_{m, h}(\epsilon, \alpha')$ as follows for a chosen value of $\epsilon > 0, \lambda > 1$ and $\alpha \in (0, 1]$.
\begin{align*}
    \beta^t_{m, h}(\epsilon, \alpha') = (R_Q+R_I)\sqrt{\lambda}+2H\sqrt{ \log\det\left(\bI + \frac{\bK^t_{ h}}{\lambda}\right) + Mt\lambda + 2M\log\left(\frac{t\cdot|\cN_\epsilon|}{\delta'}\right) + \frac{2M^2t^2\epsilon^2}{H^2\lambda}}.
\end{align*}
Then, with probability at least $1-\alpha'$, we have,
\begin{align*}
    -2\bar\beta^t_{h}\left(\epsilon, \frac{\alpha'}{M}\right)\left(\sum_{m=1}^M \left\lVert \bphi(z_m) \right\rVert_{(\bLambda^t_{m, h})^{-1}}\right) \leq \delta^t_h(\bz) \leq 0.
\end{align*}
Where $\bar\beta^t_{h}(\epsilon, \delta') = R_Q\sqrt{\lambda}+2H\sqrt{\log\det\left(\bI + \frac{\bK^t_{ h}}{\lambda}\right) + Mt(\lambda-1) + 2\log(\frac{|\cN_\epsilon|}{\delta'}) + \frac{2t^2\epsilon^2}{H^2\lambda}}$.
\end{lemma}
\begin{proof}
The proof follows the structure of the homogenous case, with a few adjustments. Assume the shorthand $\ctH = \cH \times ... \times \cH$ to denote the product of the function classes. Without loss of generality, assume that the agents are ordered with fixed indices from $1, ..., M$, and let the last global synchronization of state $h \in [H]$ be done after episode $k_t$. Consider therefore the set $\cU^m_h(t) = \left\{ \cup_{\tau=1}^{k_t} \cup_{l=1}^M (x^\tau_{l, h}, a^\tau_{l, h}, x^\tau_{l, h+1}) \right\} \bigcup \left\{ \cup_{\tau=k_t+1}^{t-1}  (x^\tau_{m, h}, a^\tau_{m, h}, x^\tau_{m, h+1}) \right\}$ for all available transitions at step $H$ for agent $m$. In this setting, instead of the original feature, we utilize the modified feature for an observation from agent $l$ defined as follows.
\begin{align}
    \bomega(x, a) &= \left[\underbrace{{\bm 0}_\cH, ..., {\bm 0}_\cH}_{(l-1)\text{ times}}, \bphi(x, a)^\top, \underbrace{{\bm 0}_\cH, ..., {\bm 0}_\cH}_{(M-l)\text{ times}} \right]^\top, \\
    \btphi(x, a) &= \bA^{- 1/2}\bomega(x, a), \text{ where, } \bA = \frac{1}{M}\left((M+1)\bI_M - {\bf 1}_M{\bf 1}^\top_M\right) \otimes \bI_d.
\end{align}
Here ${\bm 0}_\cH$ denotes the all-zeros vector in $\cH$. After each episode, each agent $m \in [M]$ therefore updates its policy parameters by solving the following kernelized ridge regression problem.
\begin{align}
    \min_{\btheta \in \ctH} L(\btheta) = \sum_{(l, (x, a, x')) \in \cU^m_h(t) \otimes [M]} \left[ r_{l, h}(x, a) + V^t_{m \rightarrow l, h+1}(x') - \left\langle \btphi(x, a), \btheta\right\rangle_{\ctH} \right]^2 + \lambda \lVert \btheta \rVert_{\ctH}^2.
\end{align}
Here, $V^t_{m \rightarrow l, h+1}$ denotes the estimate for agent $l$'s value function for step $h+1$ made by agent $m$, and the vector $\btheta$ now lies in the product space $\ctH$ instead of $\cH$. As a shorthand, let $U^m_h(t) = \left| \cU^m_h(t) \right|$ denote the size of this observation set, and without loss of generality consider that these observations are ordered as $1, ..., U^m_h(t)$. Consider now the feature matrix $\btPhi^t_{m, h} : \ctH \rightarrow \bbR^{U^m_h(t)}$ and covariance $\btLambda^t_{m, h} : \ctH \rightarrow \ctH$, given as,
\begin{align}
    \btPhi^t_{m, h} :=& \left[ \btphi(x_1, a_1)^\top, \btphi(x_2, a_2)^\top, ..., \btphi(x_{U^m_h(t)}, a_{U^m_h(t)})^\top\right]^\top, \\
    \btLambda^t_{m, h} :=& \sum_{\tau = 1}^{{U^m_h(t)}} \btphi(x_\tau, a_\tau)\btphi(x_\tau, a_\tau)^\top + \lambda \bI_\ctH = \lambda\bI_\ctH + (\btPhi^t_{m, h})^\top(\btPhi^t_{m, h}).
\end{align}
We represent the identity matrix in $\ctH$ with $\bI_{\ctH}$. The solution to the above regression problem is given as $\widehat\btheta^t_{m, h} = (\btLambda^t_{m, h})^{-1} \btPhi^t_{m, h}\ty^t_{m, h}$, where $\ty^t_{m,h}$ is the observation vector, such that $(\ty^t_{m, h})_{i} = r_{l, h}(x_i, a_i) + V^t_{m\rightarrow l, h+1}(x'_i)$ for $i \in [U^m_h(t)]$ for the corresponding agent $l$. Additionally, we have the dual-form representation~\citep{valko2013finite} of $\widehat\btheta^t_{m, h}$, given as,
\begin{align}
    \widehat\btheta^t_{m, h} = (\btLambda^t_{m, h})^{-1} \btPhi^t_{m, h}\ty^t_{m, h} = (\btPhi^t_{m, h})^\top\left(\lambda\bI + \btK^t_{m, h}\right)^{-1}\ty^t_{m, h}.
\end{align}

Where $\btK^t_{m, h}$ is the Gram matrix of observations, i.e., $\btK^t_{m, h} = \btPhi^t_{m, h}(\btPhi^t_{m, h})^\top$. Moreover, we have that,
\begin{align*}
    (\btLambda^t_{m, h})^{-1}(\btPhi^t_{m, h})^\top &= \left( (\btPhi^t_{m, h})(\btPhi^t_{m, h})^\top + \lambda\bI_\ctH\right)^{-1}(\btPhi^t_{m, h})^\top \\ &= (\btPhi^t_{m, h})^\top\left((\btPhi^t_{m, h})(\btPhi^t_{m, h})^\top + \lambda\bI\right)^{-1} \\ &= (\btPhi^t_{m, h})^\top\left(\btK^t_{m, h} + \lambda\bI\right)^{-1}.
\end{align*}
Therefore, we have, for any $z \in \cZ = \cH \times \cA$ from agent $l$,
\begin{align*}
    \btphi(z) &=  (\btLambda^t_{m, h})^{-1} \btLambda^t_{m, h} \btphi(z) \\
    &= (\btLambda^t_{m, h})^{-1}\left( (\btPhi^t_{m, h})^\top(\btPhi^t_{m, h}) + \lambda\bI_\ctH\right)\btphi(z) \\
    &= (\btLambda^t_{m, h})^{-1}(\btPhi^t_{m, h})^\top(\btPhi^t_{m, h})\btphi(z) + \lambda(\btLambda^t_{m, h})^{-1}\btphi(z) \\
    &= (\btPhi^t_{m, h})^\top\left(\btK^t_{m, h} + \lambda\bI\right)^{-1}\btk^t_{m, h}(z) + \lambda(\btLambda^t_{m, h})^{-1}\btphi(z).
\end{align*}
Where $\btk^t_{m, h} = \left[\widetilde K\left(z, (x_1, a_1)\right), ..., \widetilde K\left(z, (x_{U^t_{m, h}}, a_{U^t_{m, h}})\right)\right]$, and $\widetilde K(\cdot,\cdot) = \bomega(\cdot)^\top\bA\omega(\cdot)$. Let $\cU^t_{h} = \bigcup_{m=1}^m \bigcup_{\tau=1}^{t-1} \left\{\left(x^t_{m, h}, a^t_{m, h}, x^t_{m, h+1}\right)\right\}$ and $\left|\cU_h(t)\right| = M(t-1)$, and $\left\{\left(x_\tau, a_\tau, x'_\tau\right) \right\}_{\tau=1}^{M(t-1)}$ be an ordering of $\cU_h(t)$. Then, we define the \textit{global} bias, \textit{global} features, and \textit{global} Gram matrix respectively as,
\begin{align}
    \btk^t_{h} &= \left[\widetilde K\left(z, (x_1, a_1)\right), ..., \widetilde K\left(z, (x_{M(t-1)}, a_{M(t-1)})\right)\right] \\
    \btPhi^t_h &= \left[ \btphi(x_1, a_1)^\top, \btphi(x_2, a_2)^\top, ..., \btphi(x_{M(t-1)}, a_{M(t-1)})^\top\right]^\top\\
    \btK^t_h &= (\btPhi^t_h)(\btPhi^t_h)^\top.
\end{align}
We will be bounding the overall temporal-difference error function $\delta^t_h = \sum_{m=1}^M \delta^t_{m, h}$ in terms of the \textit{global} quantities described above. For any agent $m$, the temporal difference error in state $h$ of episode $t$ is given as,
\begin{align}
    \delta_{m, h}^t(x, a) = r_{m, h}(x, a) + \bbP_{m, h} V^t_{m, h+1} - Q^t_{m, h}(x, a) = \bbT^\star_{m, h} Q^t_{m, h+1} - Q^t_{m, h},
\end{align}
Where $\bbT^\star_{m, h}$ is the Bellman optimality operator. By Assumption~\ref{assumption:bellman_scalar} for all $(t, m, h) \in [T] \times [M] \times [H]$, since $Q^t_{m, h+1} \in [0, H]$, we have that $\bbT^\star_{m, h} Q^t_{m, h+1} \in \cQ^\star$. This implies that there exists a parameter $\bar\btheta^t_{m \rightarrow l, h} \in \cQ^\star$ such that $\bbT^\star_{l, h}Q^t_{m, h+1}(z) = \bphi(z)^\top\bar\btheta^t_{m \rightarrow l, h}$ for all $z \in \cZ$. Now, note that, for any $m \in [M], h \in [H], t \in [T], z \in \cZ$,
\begin{align}
  \bphi(z)^\top\bar\btheta^t_{m \rightarrow l, h} = (\btheta^t_{m, h})^\top\bomega(z) = (\btheta^t_{m, h})^\top\bA^{1/2}\bA^{-1/2}\bomega(z) = (\bar\btheta^t_{m, h})^\top\btphi(z).
\end{align}

Consider now the difference between the estimated Bellman operator $\btphi(z)^\top\widehat\btheta^t_{m, h}$ and the true Bellman operator $\btphi(z)^\top\bar\btheta^t_{m, h}$. We can rewrite $\bar\btheta^t_{m, h}$ as follows.
\begin{align}
    \btphi(z)^\top\bar\btheta^t_{m, h} = \btk_{m, h}^t(z)^\top \left( \btK^t_{m, h} + \lambda \bI \right)^{-1}\btPhi^t_{m, h}\bar\btheta^t_{m, h} + \lambda\cdot \btphi(z)^\top(\btLambda_{m, h}^t)^{-1}\bar\btheta^t_{m, h}
\end{align}
Additionally, we can rewrite $\widehat\btheta^t_{m, h}$ as $\btk_{m, h}^t(z)^\top \left( \btK^t_{m, h} + \lambda \bI \right)^{-1}\ty^t_{m, h}$. Therefore, we have,
\begin{align*}
    &\btphi(z)^\top\widehat\btheta^t_{m, h} - \btphi(z)^\top\bar\btheta^t_{m, h} \\
    &= \btk_{m, h}^t(z)^\top \left( \btK^t_{m, h} + \lambda \bI \right)^{-1}\left(\ty^t_{m, h} - \btPhi^t_{m, h}\bar\btheta^t_{m, h}\right) - \lambda\cdot \btphi(z)^\top(\btLambda_{m, h}^t)^{-1}\bar\btheta^t_{m, h} \\
    &\leq \underbrace{\left| \btk_{m, h}^t(z)^\top \left( \btK^t_{m, h} + \lambda \bI \right)^{-1}\left(\ty^t_{m, h} - \btPhi^t_{m, h}\bar\btheta^t_{m, h}\right) \right|}_{\text{(A)}} + \underbrace{\left|\lambda\cdot \btphi(z)^\top(\btLambda_{m, h}^t)^{-1}\bar\btheta^t_{m, h}\right|}_{\text{(B)}}
\end{align*}
We first bound term (B). By Cauchy-Schwarz, we have, since $\ctH$ is a PSD kernel,
\begin{align*}
    &\left|\lambda\cdot \btphi(z)^\top(\btLambda_{m, h}^t)^{-1}\bar\btheta^t_{m, h}\right| \\
    &\leq \left\lVert \lambda (\btLambda_{m,h}^t)^{-1}\btphi(z) \right\rVert_\ctH\cdot \left\lVert \bar\btheta^t_{m, h} \right\rVert_\ctH \\
    &= \left\lVert \lambda (\btLambda_{m,h}^t)^{-1}\btphi(z) \right\rVert_\ctH\cdot \sqrt{(\btheta^t_{m, h})^\top\bA\btheta^t_{m, h}} \\
    &= \left\lVert \lambda (\btLambda_{m,h}^t)^{-1}\btphi(z) \right\rVert_\ctH\left(\frac{1}{M}\sum_{i=1}^M\left\lVert \bar\btheta^t_{m \rightarrow i, h}\right\rVert^2_\cH + \frac{1}{M}\sum_{i=1, j=1}^{H, H} \left\lVert \bar\btheta^t_{m \rightarrow i, h}-\bar\btheta^t_{m \rightarrow j, h} \right\rVert^2_\cH\right)^{\tfrac{1}{2}} \\
    &\leq \left\lVert \lambda (\btLambda_{m,h}^t)^{-1}\btphi(z) \right\rVert_\ctH\left(R_Q + \left( \frac{1}{M}\sup_{Q : \cS \times \cA \rightarrow [0, H]} \sum_{i=1, j=1}^{H, H} \left\lVert (\bbT^\star_{i, h} - \bbT^\star_{j, h})(Q) \right\rVert^2_\cH\right)^{\tfrac{1}{2}}\right) \\
    &\leq \left\lVert \lambda (\btLambda_{m,h}^t)^{-1}\btphi(z) \right\rVert_\ctH\left(R_Q + R_I\right)\\
    &\leq \sqrt{\lambda}(R_Q + R_I)\left\lVert \btphi(z) \right\rVert_{(\btLambda^t_{m, h})^{-1}}.
\end{align*}
The first equality follows from $\bar\btheta^t_{m, h} = \bA^{\tfrac{1}{2}}\btheta^t_{m, h}$. The second equality follows from expanding $\bA^{\tfrac{1}{2}}\btheta^t_{m, h}$ and the definition of $\bA$. The second inequality follows from first applying the simple inequality $\sqrt{a+b} \leq \sqrt{a} + \sqrt{b}$, then from the fact that $\bar\btheta^t_{m \rightarrow i, h} \in \cQ^\star \implies \lVert \bar\btheta^t_{m \rightarrow n, h} \rVert_\cH \leq R_Q$, and finally using the definition of the norm $\lVert f \rVert_\cH = \sup_{f' \in \cH} \langle f, f' \rangle_{\cH}$. The third inequality follows from Assumption~\ref{assumption:bellman_hetero}, and the final inequality follows from the fact that $\btLambda^t_{m, h} \succcurlyeq \lambda \bI_{\ctH}$.

Now let us bound term (A). Let the previous synchronization step for episode $h$ be given by $k_t < t$. Therefore, any agent $m$ at time $t$ has a total of $t_{m, h} = Mk_t + (t-k_t)$ records for step $h \in [H]$. Without loss of generality, consider a permutation $\bmu$ of $[t_{m, h}]$ that maps the first $Mk_t$ elements as follows. The agent-episode pair $(n, l)$ maps to the index $i = M\cdot(l-1) + n$, and $i \in [Mk_t]$. The last $(t-k_t)$ entries of $\bmu$ refer to the observations from agent $m$ for episodes $k_t +1, ..., t$. Therefore, for each $(l, n)$ in $[M \times k_t]$ there exists a corresponding $i \in \bmu$ such that $i \leq Mk_t$ and
\begin{align}
    [\y^t_{m, t}]_i - [\btPhi^t_{m, h}\bar\btheta^t_{m \rightarrow n, h}]_i &= r_h(x^l_{n, h}, a^l_{n, h}) + V^t_{m \rightarrow n, h+1}(x^l_{n, h+1}) - \bphi(x^l_{n, h}, a^l_{n, h})^\top \bar\btheta^t_{m\rightarrow n, h} \\
    &= r_h(x^l_{n, h}, a^l_{n, h}) + V^t_{m\rightarrow n, h+1}(x^l_{n, h+1}) - \bbT^\star_{l, h}Q^t_{m\rightarrow n, h+1}(x^l_{n, h}, a^l_{n, h}) \\
    &= V^t_{m\rightarrow n, h+1}(x^l_{n, h+1}) - (\bbP_h V^t_{m\rightarrow n, h+1})(x^l_{n, h}, a^l_{n, h})
\end{align}
Furthermore, for any  $l \in [k_t + 1, t - 1]$ there exists an $i \in \bmu$ such that $i > Mk_t$ and,
\begin{align}
    [\y^t_{m, t}]_i - [\btPhi^t_{m, h}\bar\btheta^t_{m\rightarrow m, h}]_i &= r_h(x^l_{m, h}, a^l_{m, h}) + V^t_{m\rightarrow m, h+1}(x^l_{m, h+1}) - \bphi(x^l_{m, h}, a^l_{m, h})^\top \bar\btheta^t_{m\rightarrow m, h} \\
    &= r_h(x^l_{m, h}, a^l_{m, h}) + V^t_{m\rightarrow m, h+1}(x^l_{m, h+1}) - \bbT^\star_{l, h}Q^t_{m\rightarrow m, h+1}(x^l_{m, h}, a^l_{m, h}) \\
    &= V^t_{m\rightarrow m, h+1}(x^l_{m, h+1}) - (\bbP_h V^t_{m\rightarrow m, h+1})(x^l_{m, h}, a^l_{m, h})
\end{align}
Additionally, recall the reparameterization $\btk_{m, h}^t(z)^\top \left( \btK^t_{m, h} + \lambda \bI \right)^{-1} = \btphi(z)^\top(\btLambda^t_{m, h})^{-1}](\btPhi^t_{m, h})^\top$ for any $z \in \cZ$. For brevity, consider the replacement:
\begin{multline}
    \btS^t_{m, h} = \sum_{n=1}^M \sum_{\tau=1}^{k_t}\btphi(x^\tau_{n, h}, a^\tau_{n, h}) \left[V^t_{m\rightarrow n, h+1}(x^\tau_{n, h+1})- (\bbP_hV^t_{m\rightarrow n, h+1})(x^\tau_{n, h}, a^\tau_{n, h})\right] \\+ \sum_{\tau = k_t + 1}^{t-1} \btphi(x^\tau_{m, h}, a^\tau_{m, h})\left[V^t_{m\rightarrow m, h+1}(x^\tau_{m, h+1})- (\bbP_hV^t_{m\rightarrow m, h+1})(x^\tau_{m, h}, a^\tau_{m, h})\right]
\end{multline}
Replacing the above decomposition we obtain, for any $z \in \cZ$, for term (A),
\begin{align}
    \left| \btk_{m, h}^t(z)^\top \left( \btK^t_{m, h} + \lambda \bI \right)^{-1}\left(\ty^t_{m, h} - \btPhi^t_{m, h}\bar\btheta^t_{m, h}\right) \right| &= \left| \btphi(z)^\top (\btLambda^t_{m, h})^{-1}\btS^t_{m, h}\right| \\
    &\leq \left\lVert \btphi(z) \right\rVert_{(\btLambda^t_{m, h})^{-1}}\cdot \left\lVert \btS^t_{m, h} \right\rVert_{(\btLambda^t_{m, h})^{-1}}.
\end{align}
We will bound the term $ \left\lVert \btS^t_{m, h} \right\rVert_{(\btLambda^t_{m, h})^{-1}}$ by a self-normalized stochastic process concentration, and a union bound over a covering of the appropriate function class, as done in the homogenous case, albeit with some differences. Lemma~\ref{lem:beta_independent_heterogenous} provides the required bound. Lemma~\ref{lem:beta_independent_heterogenous} differs from Lemma~\ref{lem:beta_independent_centralized} in the additional factor of $M$ present in the term corresponding to the covering number. This is essentially since each agent is now simultaneously estimating all $M$ value functions for any step $h$ (which could potentially lie far apart in $\ctH$), and hence the union bound must be taken with respect to the product space of functions $\ctH = \cH^M$. Now, for each $m \in [M], t \in [T]$ and $h \in [H]$, 
\begin{align*}
    \log\det\left(\bI + \btK^t_{m, h}\right) &= \log\det\left(\bI + \sum_{z \in \cU^m_h(t)} \btphi(z)\btphi(z)^\top\right)\\
    &\leq \log\det\left(\bI + \sum_{\tau \in [t-1], m \in [M]} \btphi(x^\tau_{m, h}, a^\tau_{m, h})\btphi(x^\tau_{m, h}, a^\tau_{m, h})^\top\right)\\
    &= \log\det\left(\bI + \btK^t_{h}\right).
\end{align*}
Next, we set 
\begin{align*}
    \beta^t_{m, h}(\epsilon, \delta') = (R_Q + R_I)\sqrt{\lambda}+2H\sqrt{\cdot\log\det\left(\bI + \frac{\btK^t_{m, h}}{\lambda}\right) +Mt(\lambda-1) + 2M\log\left(\frac{t\cdot|\cN_\epsilon|}{\delta'}\right) + \frac{2M^2t^2\epsilon^2}{H^2\lambda}},
\end{align*}
and $\bar\beta^t_{h}(\epsilon, \delta') = (R_Q+R_I)\sqrt{\lambda}+2H\sqrt{ \log\det\left(\bI + \frac{\btK^t_{ h}}{\lambda}\right) + Mt\lambda + 2M\log\left(\frac{t\cdot|\cN_\epsilon|}{\delta'}\right) + \frac{2M^2t^2\epsilon^2}{H^2\lambda}}$. 

With this substitution, and a union bound, we can say that with probability at least $1-\delta'$, for any $\bz = (z_1, ..., z_M) \in \cZ^M$, we have,
\begin{align*}
    \delta^t_h(\bz) = \sum_{m=1}^M \delta^t_{m, h}(z_m) &= \sum_{m=1}^M \btphi(z_m)^\top\widehat\btheta^t_{m, h} - \btphi(z_m)^\top\bar\btheta^t_{m, h} \\
    &\leq \sum_{m=1}^M \left( \left\lVert \btphi(z_m) \right\rVert_{(\bLambda^t_{m, h})^{-1}}\left(R_Q\sqrt{\lambda} + \left\lVert \btS^t_{m, h} \right\rVert_{(\btLambda^t_{m, h})^{-1}}\right) \right)\\
    &\leq \sum_{m=1}^M \left( \beta^t_{m, h}\left(\epsilon, \frac{\delta'}{M}\right)\left\lVert \btphi(z_m) \right\rVert_{(\btLambda^t_{m, h})^{-1}}\right) \\
    &\leq \bar\beta^t_{m, h}\left(\epsilon, \frac{\delta'}{M}\right)\left(\sum_{m=1}^M \left\lVert \btphi(z_m) \right\rVert_{(\btLambda^t_{m, h})^{-1}}\right).
\end{align*}
Here, the first equality follows from the independence of the environments, and the second inequality follows by first applying Lemma~\ref{lem:beta_independent_heterogenous} with probability $\delta'/M$ to each of the $M$ terms, and then applying a union bound over all the agents. Finally, we obtain the final form of the proof by the following decomposition.
\begin{align*}
    -\delta^t_h(\bz) &= \sum_{m=1}^M \left[Q^t_{m, h}(z_m) - \bphi(z_m)^\top\bar\btheta^t_{m, h}\right] \\
    &\leq \sum_{m=1}^M \bphi(z_m)^\top\left[ \widehat\btheta^t_{m, h} - \bar\btheta^t_{m, h}\right] + \bar\beta^t_{h}\left(\epsilon, \frac{\alpha'}{M}\right)\left(\sum_{m=1}^M \left\lVert \bphi(z_m) \right\rVert_{(\bLambda^t_{m, h})^{-1}}\right) \\
    &\leq 2\bar\beta^t_{h}\left(\epsilon, \frac{\alpha'}{M}\right)\left(\sum_{m=1}^M \left\lVert \bphi(z_m) \right\rVert_{(\bLambda^t_{m, h})^{-1}}\right).
\end{align*}
Here, the first inequality is true from the algorithm itself, and the second inequality holds with probability at least $1-\alpha'$.
\end{proof}

\begin{lemma}
For any $m \in [M], h \in [H]$ and $t \in [T]$, let $k_t$ denote the episode after which the last global synchronization has taken place, and $\btS^t_{m, h}$ and $\btLambda^k_t$ be defined as follows.
\begin{multline*}
    \btS^t_{m, h} = \sum_{n=1}^M \sum_{\tau=1}^{k_t}\btphi(x^\tau_{n, h}, a^\tau_{n, h}) \left[V^t_{m\rightarrow n, h+1}(x^\tau_{n, h+1})- (\bbP_hV^t_{m\rightarrow n, h+1})(x^\tau_{n, h}, a^\tau_{n, h})\right] \\+ \sum_{\tau = k_t + 1}^{t-1} \btphi(x^\tau_{m, h}, a^\tau_{m, h})\left[V^t_{m\rightarrow n, h+1}(x^\tau_{m, h+1})- (\bbP_hV^t_{m\rightarrow n, h+1})(x^\tau_{m, h}, a^\tau_{m, h})\right],
\end{multline*} 
\begin{align*}
    \btLambda^k_t = \sum_{n=1}^M \sum_{\tau=1}^{k_t}\btphi(x^\tau_{n, h}, a^\tau_{n, h})\btphi(x^\tau_{n, h}, a^\tau_{n, h})^\top + \sum_{\tau = k_t + 1}^{t-1}  \btphi(x^\tau_{m, h}, a^\tau_{m, h})\btphi(x^\tau_{m, h}, a^\tau_{m, h})^\top + \lambda\bI_\ctH.
\end{align*}
Then, with probability at least $1-\delta$,
\begin{align*}
    \left\lVert \btS^t_{m, h} \right\rVert_{(\btLambda^t_{m, h})^{-1}} &\leq 2H\sqrt{ \log\det\left(\bI + \frac{\bK^t_{m, h}}{\lambda}\right) + Mt(\lambda-1) + 2M\log\left(\frac{t\cdot|\cN_\epsilon|}{\delta}\right) + \frac{2M^2t^2\epsilon^2}{H^2\lambda}}.
\end{align*}
where $\cN_\epsilon$ denotes an $\epsilon-$covering of $\cV_{\text{UCB}}$, and $\bK^t_{m, h} = (\btPhi^t_{m, h})(\btPhi^t_{m, h})^\top$ is the Gram matrix estimate of agent $m$.
\label{lem:beta_independent_heterogenous}
\end{lemma}
\begin{proof}
The proof in this case follows the structure of the homogenous independent case with careful modifications. Consider the family of value functions $\cV_{\text{UCB}}$ that contains each of the functions expressed by the UCB value iteration in the heterogenous algorithm. Furthermore, consider the following function defined over $(x, l) \in \cS \times [M]$:
\begin{align}
    V^t_{m, h}(x, l) &= \sum_{n=1}^M \bone\left\{l = n\right\} \cdot V^t_{m \rightarrow l, h}(x).
\end{align}
Next, consider $\cV'_{\text{UCB}} = \left\{ V(x, y) = \sum_{i=1}^M \bone\left\{i = y\right\}V_i(x) : V_i \in \cV_{\text{UCB}}\ \forall \ i \in [M]\right\}$ as a function class over all multiagent value functions. Next, consider the following quantity that characterizes a distance between two multi-agent value functions for any specific agent $l$.
\begin{align}
    \text{dist}_M(V, V') = \sup_{x \in \cS, l \in [M]}|V(x, l) - V'(x, l)|.
\end{align}
Observe that $\btS^t_{m, h}$ can be rewritten in terms of $V^t_{m, h}$.
\begin{multline}
     \btS^t_{m, h} = \sum_{n=1}^M \sum_{\tau=1}^{k_t}\btphi(x^\tau_{n, h}, a^\tau_{n, h}) \left[V^t_{m, h+1}(x^\tau_{n, h+1}, n)- (\bbP_hV^t_{m, h+1})(x^\tau_{n, h}, a^\tau_{n, h}, n)\right] \\+ \sum_{\tau = k_t + 1}^{t-1} \btphi(x^\tau_{m, h}, a^\tau_{m, h})\left[V^t_{m, h+1}(x^\tau_{m, h+1}, m)- (\bbP_hV^t_{m, h+1})(x^\tau_{m, h}, a^\tau_{m, h}, m)\right].
\end{multline}Now, our goal is to bound the following quantity for any $V^t_{m, h} \in \cV'_{\text{UCB}}$.
\begin{align}
    \left\lVert \btS^t_{m, h} \right\rVert_{(\bLambda^t_{m, h})^{-1}} &\leq \sup_{V \in \cV'_{\text{UCB}}}\left\lVert \btS^t_{m, h} \right\rVert_{(\bLambda^t_{m, h})^{-1}}
\end{align}
Our approach here onwards is similar to the homogenous case. Let $\cN'_\epsilon$ be an $\epsilon-$covering of $\cV'_{\text{UCB}}$ with respect to the distance mentioned above. Our first step is to demonstrate that $|\cN'_\epsilon| \leq |\cN_\epsilon|^M$, where $\cN_\epsilon$ is an $\epsilon-$covering of $\cV_{\text{UCB}}$. Let $\cN_\epsilon$ be an $\epsilon-$covering of $\cV'_{\text{UCB}}$. Consider the set of functions $\widetilde\cV = \left\{ V(x, y) = \sum_{i=1}^M \bone\left\{i = y\right\}V_i(x) : V_i \in \cN_\epsilon\ \forall \ i \in [M]\right\}$. For every $V \in \cV'_{\text{UCB}}$, we have that,
\begin{align}
    V(x, y) = \sum_{n=1}^M\bone\left\{y = n\right\}V_n(x)
\end{align}
Where $V_1, ..., V_M$ are elements of $\cV_{\text{UCB}}$. Therefore, by the definition of $\cN_\epsilon$, there exists a sequence $V'_1, V'_2, ..., V'_M$ where $V'_i \in \cN_\epsilon$ such that $\sup_{x \in \cS}\left| V_i(x) - V'_i(x) \right| \leq \epsilon$. By selecting $V'_1, ..., V'_M$ from $\cN_\epsilon$, we therefore know that by construction there always exists $V' \in \widetilde\cV$ such that $\sup_{x \in \cS, y \in [M]} \left| V(x, y) - V'(x, y) \right| \leq \epsilon$. Therefore $\widetilde\cV$ is an $\epsilon$-covering of $\cV'_{\text{UCB}}$ under $\text{dist}_M$, and hence $|\cN'_\epsilon| \leq |\widetilde\cV|$. Now, each element in the finite set $\widetilde\cV$ can be described by at most $M$ distinct elements of $\cN_\epsilon$, and hence there can be at most $|\cN_\epsilon|^M$ unique elements in $\widetilde\cV$. Therefore, $|\cN'_\epsilon| \leq |\widetilde\cV| \leq |\cN_\epsilon|^M$.

Now, we have that since $\cN'_\epsilon$ is a covering of $\cV'_{\text{UCB}}$ then there exists a $V' \in \cN'_\epsilon$ such that $\text{dist}_M(V, V') \leq \epsilon$ for every $V \in \cV'_{\text{UCB}}$. Then, we have by the fact that $(a+b)^2 \leq 2a^2 + 2b^2$,
\begin{align}
    \sup_{V \in \cV'_{\text{UCB}}}\left\lVert \btS^t_{m, h} \right\rVert^2_{(\bLambda^t_{m, h})^{-1}} \leq 2\sup_{V \in \cN'_\epsilon}\left\lVert \btS^t_{m, h} \right\rVert^2_{(\bLambda^t_{m, h})^{-1}} + \frac{8t^2M^2\epsilon^2}{\lambda}.
    \label{eqn:s_covering_split_hetero}
\end{align}
To bound the first quantity on the RHS, note that the function $V^t_{m, h+1}$ for all $n \in [M]$ depends on the history from all $M$ agents from the first $k_t$ episodes, and the personal historical data for the first $(t-1)$ episodes, and hence depends on 
\begin{align*}
    \left(\cup_{n \in [M], \tau \in [k_t]}\{(x^\tau_{n, h}, a^\tau_{n, h}, x^\tau_{n, h+1})\}\right) \bigcup \left(\cup_{\tau \in [k_t+1, t-1} \{(x^\tau_{m, h}, a^\tau_{m, h}, x^\tau_{m, h+1})\}\right)
\end{align*}
Further, note that for some $t \in [T]$, $k_t$ is fixed and known \textit{a priori}, i.e., $k_t \leq t$. To bound the term we will construct an appropriate filtration to use the self-normalized concentration. We highlight that in the multi-agent case with stochastic communication, it is not straightforward to provide a uniform martingale concentration that holds for all $t \in [T]$ simultaneously (as is done in the single-agent case), as the stochasticity in the environment dictates when communication will take place, and subsequently the quantity considered within self-normalization will depend on this communication itself. To circumvent this issue, we will first fix $k_t \leq t$ and obtain a filtration for a fixed $k_t$. Then, we will take a union bound over all $k_t \in [t]$ to provide the final self-normalized bound. We first fix $k_t$ as a constant quantity known \textit{a priori}, and define the following mappings where $i \in \left[M(t-1)\right], l \in [t-1], $ and $n \in [M]$.
\begin{align*}
    \mu(i) = \left\lceil \frac{i}{M} \right\rceil, 
    \nu(i) = i (\text{mod } M), \text{ and, }
    \eta(l, n) = l\cdot(M+1) + n - 1.
\end{align*}  
Now, consider the stochastic processes $\{\tilde x_\tau\}_{\tau = 1}^\infty$ and $\{\widehat\bphi_\tau\}_{\tau = 1}^\infty$, where $\tilde x_i = x^{\nu(i)}_{\mu(i), h+1}$ and,
\begin{align*}
    \widehat \bphi_i = \btphi\left(x^{\nu(i)}_{\mu(i), h}, a^{\nu(i)}_{\mu(i), h}\right)\otimes \bone_\ctH\left\{ \left(\mu(i) = m\right) \lor \left(\nu(i) \leq k_t\right)\right\}
\end{align*} 
Here $\otimes$ denotes the Hadamard product, and $\bone_{\ctH}$ is the indicator function in $\ctH$. Consider the filtration $\{\cF_\tau\}_{\tau=0}^\infty$, where $\cF_0$ is empty, and $\cF_\tau = \sigma\left(\left\{ \bigcup (\tilde x_i, \widehat\bphi_i)\right\}_{i \leq \tau}\right)$, where $\sigma(\cdot)$ denotes the $\sigma-$algebra formed by a finite set.

At any instant $t$ for any agent $m$, the function $V^t_{m, h+1}$ and features $\btphi(x^t_{m, h}, a^t_{m, h})$ depend only on historical data from all other agents $[M] \setminus \{m\}$ up to the last episode of synchronization $k_t \leq t - 1$ and depend on the personal data up to episode $t-1$. Hence, both are $V^t_{m, h+1}$ and $\bphi(x^t_{m, h}, a^t_{m, h})$ are measurable with respect to 
\begin{align*}
    \sigma\left(\left\{ \bigcup_{l=1}^{k_t}\bigcup_{n=1}^{M} (\tilde x_{\eta(l, n)}, \tilde \bphi_{\eta(l, n)})\right\} \bigcup \left\{\bigcup_{l=k_t+1}^{t-1} (\tilde x_{\eta(l, m)}, \tilde\bphi_{\eta(l, m)})\right\} \right),
\end{align*}
which is a subset of $\cF_{\eta(t, m)}$. Therefore $V^t_{m, h+1}$ is $\cF_{\eta(t, m)}-$measurable. Note that $\widehat\bphi_{m, h}(i)$ depends on the original feature $\btphi$ and the indicator function depending on $m, \mu(i), \nu(i)$ and $t_{s,h}$, all of which are $\cF_i-$measurable if $k_t$ is fixed in advance. Therefore $\widehat\bphi_{m, h}(i)$ is also $\cF_i-$measurable. We therefore have that, for any value function $V \in \cV'_{\text{UCB}}$,
\begin{align*}
    &\sum_{\tau=1}^{M(t-1)} \widehat\bphi_{m, h}(\tau)\left\{ V(\tilde x_\tau, \mu(\tau)) - \bbE[V(\tilde x_\tau, \mu(\tau)) | \cF_{\tau-1}] \right\} \\
    &= \sum_{\tau=1}^{M(t-1)} \left[\widehat\bphi_\tau\otimes \bone_\ctH\left\{ \left(\mu(\tau) = m\right) \lor \left(\nu(\tau) \leq k_t\right)\right\}\right]\left\{ V(\tilde x_\tau, \mu(\tau)) - \bbE\left[V(\tilde x_\tau, \mu(\tau)) | \cF_{\tau-1}\right] \right\} \\
    &= \sum_{(l_\tau, (x_\tau, a_\tau, x'_\tau)) \in \cU^m_h(t)} \widehat\bphi(x_\tau, a_\tau)\left\{ V(x'_\tau, l_\tau) - \bbE[V(x'_\tau, l_\tau) | \cF_{\tau-1}] \right\}. 
\end{align*}
Next, consider $\widehat\bLambda^t_{m, h} = \lambda \bI_d + \sum_{\tau=1}^{M(t-1)} \widehat\bphi_{m, h}(\tau)\widehat\bphi_{m, h}(\tau)^\top$. For the second term, we have,
\begin{align*}
     \widehat\bLambda^t_{m, h} &= \lambda \bI_d +\sum_{\tau=1}^{M(t-1)} \widehat\bphi_{m, h}(\tau)\widehat\bphi_{m, h}(\tau)^\top \\
     &=\lambda \bI_d +\sum_{(l_\tau, (x_\tau, a_\tau, x'_\tau)) \in\cU^m_h(t)} \btphi(x_\tau, a_\tau)\btphi(x_\tau, a_\tau)^\top = \btLambda^t_{m, h}.
\end{align*}
We will bound $\left\lVert \sum_{\tau=1}^{M(t-1)} \widehat\bphi_{m, h}(\tau)\left\{V^t_{h, m+1}(\tilde x_\tau, \mu(\tau)) - \bbE[V^t_{h, m+1}(\tilde x_\tau, \mu(\tau)) | \cF_{\tau-1}]\right\} \right\rVert_{(\widehat\bLambda^t_{m, h})^{-1}}$, which by the relationship above will bound the required quantity $\left\lVert \btS^t_{m, h} \right\rVert_{(\btLambda^t_{m, h})^{-1}}$ for a fixed $t_{s,h}$ and taking a union bound over all $k_t \leq t$ will bound the overall quantity. We proceed following a self-normalized martingale bound and a covering argument. Applying Lemma~\ref{lem:self_normalized_single_task_hetero} to  $\left\lVert \sum_{\tau=1}^{M(t-1)} \widehat\bphi_{m, h}(\tau)\left\{V^t_{h, m+1}(\tilde x_\tau, \mu(\tau)) - \bbE[V^t_{h, m+1}(\tilde x_\tau, \mu(\tau)) | \cF_{\tau-1}]\right\} \right\rVert_{(\widehat\bLambda^t_{m, h})^{-1}}$ under the filtration $\{\cF_\tau\}_{\tau=0}^\infty$ described earlier, we have that with probability at least $1-\delta'$,
\begin{align*}
    &\sup_{V \in \cN'_\epsilon} \left\lVert \btS^t_{m, h} \right\rVert^2_{(\btLambda^t_{m, h})^{-1}} \\
    &= \sup_{V \in \cN'_\epsilon}\left\lVert \sum_{\tau=1}^{M(t-1)} \widehat\bphi_{m, h}(\tau)\left\{V^t_{h, m+1}(\tilde x_\tau, \mu(\tau)) - \bbE[V^t_{h, m+1}(\tilde x_\tau, \mu(\tau)) | \cF_{\tau-1}]\right\} \right\rVert^2_{(\widehat\bLambda^t_{m, h})^{-1}} \\
    &\leq 4H^2\cdot\log\det\left(\bI + \frac{\widehat\bK^t_{m, h}}{\lambda}\right) + 4H^2Mt(\lambda-1) + 8H^2\log\left(\frac{|\cN'_\epsilon|}{\delta'}\right) + \frac{8M^2t^2\epsilon^2}{\lambda}.
\end{align*}
Where $[\widehat\bK^t_{m, h}]_{i, j} = \widehat\bphi_i^\top\widehat\bphi_j$ is the Gram matrix of observations available to agent $m$ for state $h$ at episode $t$. Now, note that for any $i, j \in [M(t-1)]$ such that $(x^{\nu(i)}_{\mu(i), h}, a^{\nu(i)}_{\mu(i), h}) \not\in \cU^m_h(t)$ and $(x^{\nu(j)}_{\mu(j), h}, a^{\nu(j)}_{\mu(j), h}) \not\in \cU^m_h(t)$, $[\widehat\bK^t_{m, h}]_{i, j} = 0$. Therefore, $\widehat\bK^t_{m, h} = \widetilde\bK^t_{m, h}$. Therefore, we have that, with probability at least $1-\delta'$, for a fixed $k_t \leq t$, since $|\cN'_\epsilon| \leq |\cN_\epsilon|^M$,
\begin{align*}
   \sup_{V \in \cN'_\epsilon}  \left\lVert \btS^t_{m, h} \right\rVert_{(\btLambda^t_{m, h})^{-1}} &\leq 2H\sqrt{ \log\det\left(\bI + \frac{\bK^t_{m, h}}{\lambda}\right) + Mt(\lambda-1) + 2M\log\left(\frac{|\cN_\epsilon|}{\delta}\right) + \frac{2M^2t^2\epsilon^2}{H^2\lambda}}.
\end{align*}
Taking a union bound over all $k_t \leq t$, we have that, with probability at least $1-\delta'$, 
\begin{align*}
   \sup_{V \in \cN'_\epsilon}  \left\lVert \btS^t_{m, h} \right\rVert_{(\btLambda^t_{m, h})^{-1}} &\leq 2H\sqrt{ \log\det\left(\bI + \frac{\bK^t_{m, h}}{\lambda}\right) + Mt(\lambda-1) + 2M\log\left(\frac{t\cdot|\cN_\epsilon|}{\delta}\right) + \frac{2M^2t^2\epsilon^2}{H^2\lambda}}.
\end{align*}
Replacing this bound in Equation~(\ref{eqn:s_covering_split_hetero}) gives us the final result.
\end{proof}
\begin{lemma}
\label{lem:self_normalized_single_task_hetero}
\end{lemma}
\begin{proof}

\end{proof}

\begin{lemma}[Variance control via communication in heterogeneous factored environments]
Let Algorithm~\ref{alg:centralized_independent_hetero} be run for any $T > 0$ and $M \geq 1$, with $S$ as the communication control factor. Then, the following holds for the cumulative variance for any RKHS $\cH$ defined by kernel $K$ for any $\omega > 1$.
\begin{align}
    \sum_{m=1}^M\sum_{t=1}^T \left\lVert \bphi(z^t_{m, h}) \right\rVert_{(\bLambda^t_{m, h})^{-1}} \leq \left(  \frac{2\Gamma_K(MT, \lambda)}{\log \omega} \right)M\sqrt{S} + \omega\sqrt{2MT\Gamma_K(MT, \lambda)}.
\end{align}
\label{lem:sum_variance_homo}
Here $\Gamma_K(T, \lambda)$ is the cumulative information gain defined in Definition~\ref{def:infogain_homo}.
\end{lemma}
\begin{proof}
The key challenge to bounding this quantity is that the communication protocol depends on $\cH$ as well. We first assume that $\cH$ is finite-dimensional (i.e., $d_\cH < \infty$), and tackle the infinite case later. Consider the following mappings $\nu_M, \nu_T : [MT] \rightarrow [M] \times [T]$.
\begin{align}
    \nu_M(\tau) = \tau (\text{mod } M), \text{and } \nu_T = \left\lceil \frac{\tau}{M}\right\rceil.
\end{align}
Now, consider the quantity $\bar\bLambda^\tau_h = \lambda\bI_d + \sum_{u=1}^\tau \bphi\left(z^{\nu_T(u)}_{\nu_M(u), h}\right)\bphi\left(z^{\nu_T(u)}_{\nu_M(u), h}\right)^\top$ for $\tau > 0$ and $\bar\bLambda^0_h = \lambda\bI_d$. Furthermore, assume that global synchronization for step $h$ occurs at round $\bsigma_h = (\sigma_{1, h}, ..., \sigma_{N, h})$ where there are a total of $N-1$ rounds of synchronization and $\sigma_{i, h} \in [T] \forall h \in [H], i \in [N-1]$ and $\sigma_{N, h} = T$, i.e., the final round. We have that $\det(\bar\bLambda^0_h) = \lambda$ and $\det(\bar\bLambda^{MT}_h)  = \det(\lambda\bI +\bK^t_h)$. Thus, for any $\omega > 1$,
\begin{align}
    \log_\omega\left(\frac{\det(\bar\bLambda^{MT}_h)}{\det(\bar\bLambda^0_h)}\right) \leq \log_\omega\det\left(\bI +\frac{\bK^t_h}{\lambda}\right).
\end{align}
Let $R_h = \left\lceil  \log_\omega\det\left(\bI +\frac{\bK^T_h}{\lambda}\right) \right\rceil$. It follows that there exist at most $R_h$ periods between synchronization (i.e., intervals $\sigma_{k-1}$ to $\sigma_k$ for $k \in [N]$) in which the following does not hold true:
\begin{align}
    1 \leq \frac{\det(\bar\bLambda^{\sigma_k}_h)}{\det(\bar\bLambda^{k-1, h}_h)}\leq \omega.
    \label{eqn:interval_sync_single_agent}
\end{align}
Let us denote the event when Equation~(\ref{eqn:interval_sync_single_agent}) does holds for an interval $\sigma_{k-1}$ to $\sigma_k$ as $E$. Now, for any $t \in [\sigma_{k-1}, \sigma_k]$, we have, for any $m \in [M]$,
\begin{align}
    \left\lVert \bphi(z^t_{m, h}) \right\rVert_{(\bLambda^t_{m, h})^{-1}} &\leq \left\lVert \bphi(z^t_{m, h}) \right\rVert_{(\bar\bLambda^{t}_{h})^{-1}}\sqrt{\frac{\det\left(\bar\bLambda^t_{h}\right)}{\det\left(\bLambda^t_{m,h}\right)}} \\
    &\leq \left\lVert \bphi(z^t_{m, h}) \right\rVert_{(\bar\bLambda^t_{h})^{-1}}\sqrt{\frac{\det\left(\bar\bLambda^{\sigma_k}_{ h}\right)}{\det\left(\bar\bLambda^{\sigma_{k-1}}_{h}\right)}} \\
    &\leq \omega\left\lVert \bphi(z^t_{m, h}) \right\rVert_{(\bar\bLambda^{t}_{h})^{-1}}.
\end{align}
Here, the first inequality follows from the fact that $\bLambda^t_{m, h} \preccurlyeq \bar\bLambda^t_{h}$, the second inequality follows from the fact that $\bLambda^t_{m, h} \preccurlyeq \bar\bLambda^{\sigma_k}_{h} \implies \det(\bLambda^t_{m, h}) \leqslant \det(\bar\bLambda^{\sigma_k}_{h})$, and $\bLambda^t_{m, h} \succcurlyeq \bar\bLambda^{\sigma_{k-1}}_{h} \implies \det(\bLambda^t_{m, h}) \geqslant \det(\bar\bLambda^{\sigma_{k-1}}_{h})$; and the final inequality follows from the fact that event $E$ holds. Now, we can consider the partial sums only in the intervals for which event $E$ holds. For any $t \in [T]$, consider $\sigma(t) = \max_{i \in [N]} \{\sigma_{i, h} | \sigma_{i, h} \leq t\}$ denote the last round of synchronization prior to episode $t$. We have that,
\begin{align}
    \sum_{t: E\text{ is true}}^T\sum_{m=1}^M \left\lVert \bphi(z^t_{m, h}) \right\rVert_{(\bLambda^t_{m, h})^{-1}} &\leq \sqrt{MT\sum_{m=1}^M\sum_{t: E\text{ is true}}^T \left\lVert \bphi(z^t_{m, h}) \right\rVert^2_{(\bLambda^t_{m, h})^{-1}}} \\
    &\leq \omega\sqrt{MT\sum_{m=1}^M\sum_{t: E\text{ is true}}^T \left\lVert \bphi(z^t_{m, h}) \right\rVert^2_{(\bar\bLambda^t_{h})^{-1}}}\\
    &\leq \omega\sqrt{MT\sum_{m=1}^M\sum_{t=1}^T \left\lVert \bphi(z^t_{m, h}) \right\rVert^2_{(\bar\bLambda^t_{h})^{-1}}}\\
    &=\omega\sqrt{MT\sum_{m=1}^M\sum_{\tau=1}^T \left\lVert \bphi(z^{\nu_T(\tau)}_{\nu_M(\tau), h}) \right\rVert^2_{(\bar\bLambda^t_{h})^{-1}}} \\
    &= \omega\sqrt{MT\log\det\left(\bI +\frac{\bK^T_h}{\lambda}\right)}.
\end{align}
Here, the first inequality follows from Cauchy-Schwarz, the second inequality follows from the fact that event $E$ holds, and the final equality follows from Lemma~\ref{lem:variance_sum} for any $\omega > 1$. Now, we sum up the cumulative sum for episodes when $E$ does not hold. Consider an interval $\sigma_{k-1}$ to $\sigma_k$ for $k \in [N]$ of length $\Delta_{k, h} = \sigma_k - \sigma_{k-1}$ in which $E$ does not hold. We have that,
\begin{align}
    \sum_{m=1}^M\sum_{t=\sigma_{k-1}}^{\sigma_k} \left\lVert \bphi(z^t_{m, h}) \right\rVert_{(\bLambda^t_{m, h})^{-1}} &\leq \sum_{m=1}^M\sqrt{\Delta_{k, h}\sum_{t=\sigma_{k-1}}^{\sigma_k} \left\lVert \bphi(z^t_{m, h}) \right\rVert^2_{(\bLambda^t_{m, h})^{-1}}} \\
    &\leq \sum_{m=1}^M\sqrt{\Delta_{k, h}\cdot \log_\omega\left(\frac{\det(\bLambda^{\sigma_k}_{m, h})}{\det(\bLambda^{\sigma_{k-1}}_{m, h})}\right)} \\
    &\leq \sum_{m=1}^M\sqrt{\Delta_{k, h}\cdot \log_\omega\left(\frac{\det(\bar\bLambda^{\sigma_k}_{ h})}{\det(\bar\bLambda^{\sigma_{k-1}}_{ h})}\right)} \\
    &\leq M\sqrt{S}.
\end{align}
The last inequality follows from the synchronization criterion. Now, note that there are at most $R_h$ periods in which event $E$ does not hold, and hence the total sum in this period can be bound as,
\begin{align}
    \sum_{m=1}^M\sum_{t : E \text{ is not true}}^T \left\lVert \bphi(z^t_{m, h}) \right\rVert_{(\bLambda^t_{m, h})^{-1}} &\leq R_hM\sqrt{S} \\
    &\leq \left(  \log_\omega\det\left(\bI +\frac{\bK^T_h}{\lambda}\right) + 1\right)M\sqrt{S}.
\end{align}
Therefore, we can bound the total variance as,
\begin{align*}
    &\sum_{m=1}^M\sum_{t=1}^T \left\lVert \bphi(z^t_{m, h}) \right\rVert_{(\bLambda^t_{m, h})^{-1}} \\ 
    &\leq  \left(  \log_\omega\det\left(\bI +\frac{\bK^T_h}{\lambda}\right) + 1\right)M\sqrt{S} + \omega\sqrt{MT\log\det\left(\bI +\frac{\bK^T_h}{\lambda}\right)} \\
    &\leq  \left(  \frac{2\Gamma_K(T, \lambda)}{\log \omega} \right)M\sqrt{S} + \omega\sqrt{2MT\Gamma_K(T, \lambda)}.
\end{align*}
\end{proof}

\begin{lemma}
For $ \xi_{t, m, h}^1$ and $ \xi_{t, m, h}^2$ as defined earlier and any $\delta \in (0, 1)$, we have with probability at least $1-\delta/2$,
\begin{align}
\sum_{t=1}^T \sum_{m=1}^M\sum_{h=1}^H \left( \xi_{t, m, h}^1 + \xi_{t, m, h}^2 \right) \leq \sqrt{16H^3MT\log\left(\frac{4}{\delta}\right)}.
\end{align}
\label{lem:martingale_independent}
\end{lemma}
\begin{proof}
We generalize the procedure from~\cite{jin2018q}, by demonstrating that the overall sums can be written as bounded martingale difference sequences with respect to an appropriately chosen filtration. For any $(t, m, h) \in [T] \times [M] \times [H]$, we define $\sigma$-algebras $\cF_{t, m, h, 1}$ and $\cF_{t, m, h, 2}$ as,
\begin{align}
    \cF_{t, m, h, 1}  &= \sigma\left(\left\{ \left(x^\tau_{l, i}, a^\tau_{l, i}\right)\right\}_{(\tau, l, i) \in [t-1]\times [M] \times [H]} \cup \left\{ \left(x^t_{l, i}, a^t_{l, i}\right)\right\}_{(i, l) \in [h] \times [m-1]} \cup \left\{ \left(x^t_{m, i}, a^t_{m, i}\right)\right\}_{i \in [h]} \right),\\
    \cF_{t, m, h, 2}  &= \sigma\Big(\left\{ \left(x^\tau_{l, i}, a^\tau_{l, i}\right)\right\}_{(\tau, l, i) \in [t-1]\times [M] \times [H]} \cup \left\{ \left(x^t_{l, i}, a^t_{l, i}\right)\right\}_{(i, l) \in [h] \times [m-1]} \cup \left\{ \left(x^t_{m, i}, a^t_{m, i}\right)\right\}_{i \in [h]} \cup \left\{ x^t_{m, h+1}\right\} \Big).
\end{align}
Where we denote the $\sigma-$algebra generated by a finite set by $\sigma(\cdot)$. For any $t \in [T], m \in [M], h \in [H]$, we can define the timestamp index $\tau(t, m, h, k)$ as,
\begin{align}
    \tau(t, m, h, k) = (t-1)\cdot2HM + 2h(m-1) + (h-1)\cdot 2 + k,
\end{align}
Following~\cite{jin2018q} we see that this ordering ensures that the $\sigma-$algebras from earlier form a filtration. We can see that for any agent $m \in [M]$, $Q^t_{m, h}$ and $V^t_{m, h}$ are both obtained based on the trajectories of the first $(t-1)$ episodes, and are both measurable with respect to $\cF_{t, 1, 1, 1}$ (which is a subset of $\cF_{t, m, h, k}$ for all $h \in [H]$, $m \in [M]$ and $k \in [2]$). Moreover, note that $a^t_{m, h} \sim \pi_{m, t}(\cdot | x^t_{m, h})$ and $x^t_{m, h+1} \sim \bbP_{m, h}(\cdot | x^t_{m, h}, a^t_{m, h})$. Therefore,
\begin{align}
    \bbE_{\pi_{m, t}}[\xi_{t, m, h}^1 | \cF_{t, m, h-1, 2}]  = 0 \text{ and, }
 \bbE_{\bbP_{m, h}}[\xi_{t, m, h}^2 | \cF_{t, m, h, 1}] =  0.
\end{align}
where we identify $\cF_{t, m, 0, 2}$ with $\cF_{t-1, m, H, 2}$ for all $t \geq 2$ and $m \in [M]$ and set $\cF_{1, 0, 0, 2}$ with the empty set. Finally, we can define the martingale $\{U_{t, m, h, k}\}_{(t, h, m) \in [T]\times[M]\times[H]\times[2]}$ indexed by $\tau(t, m, h, k)$ defined earlier, as follows. For any $(t, m, h, k) \in [T] \times [M] \times [H] \times [2]$, we define
\begin{align}
    U_{t, m, h, k} =\left\{ \sum_{(a,b,c, d)} \xi^d_{a, b, c} : \tau(a, b, c, d) \leq \tau(t, m, h, k)\right\},
\end{align}
Additionally, we have that
\begin{align}
    U_{T, M, H, 2} &= \sum_{t=1}^T \sum_{m=1}^M \sum_{h=1}^H \left( \xi_{t, m, h}^1 + \xi_{t, m, h}^2 \right).
\end{align}
Now, we have that for each $m \in \cM$, $V^t_{m, h}, Q^t_{m, h}, V^{\pi_{m, t}}_{m, h}, Q^{\pi_{m, t}}_{m, h}$ take values in $[0, H]$. Therefore, wh have that $ \xi_{t, m, h}^1 \leq 2H$ and $\xi_{t, h}^2 \leq 2H$ for all $(t, m, h) \in [T] \times [M] \times [H]$. This allows us to apply the Azuma-Hoeffding inequality~\citep{azuma1967weighted} to $U_{T, M, H, 2}$. We therefore obtain that for all $\tau > 0$,
\begin{align}
    \bbP\left( \sum_{t=1}^T \sum_{m=1}^M \sum_{h=1}^H \left( \xi_{t, h}^1 + \xi_{t, h}^2 \right) > \tau \right) \leq 2\exp\left(\frac{-\tau^2}{16H^3MT}\right).
\end{align}
Setting the RHS as $\delta/2$,we obtain that with probability at least $1-\delta/2$,
\begin{align}
    \sum_{t=1}^T \sum_{m=1}^M \sum_{h=1}^H \left( \xi_{t, m, h}^1 + \xi_{t, m, h}^2 \right) \leq \sqrt{16H^3MT\log\left(\frac{4}{\delta}\right)}.
\end{align}
\end{proof}
